# Supplementary material for: Random Forest Regression Feature Importance for Climate Impact Pathway Detection
Source: arXiv:2409.16609 source file (2024-12-25)
Supplement: Supplementary file 1 [file appendices.tex]

\section*{Appendix}

Here we present the full, unpruned, pathway results so the reader can see different impact pathways that could be derived using more or less strict pruning criteria. 
% \mglbnote{This may be way too much extra information, all 4 tables take up 43 pages (10-15 pages per table). I tried to reduce the space between lines in the long tables, but I couldn't figure out how to make the tables more compact than this.}

\subsection*{A.1.  Global Stratosphere}

\begin{longtblr}[
  caption = {Mount Pinatubo exemplar: unpruned pathway edge weights and their standard deviations for the stratospheric warming pathway obtained using globally-averaged data windowed to 750 days.},
  label = {tab:app_global_strat},
]{
  colspec = {llcccc},
  width=\textwidth,
  rowsep=0pt,
  cells={font=\small},
  rowhead = 2,
} 

    \hline \hline
        \multirow{2}{*}{\textbf{Source}} & \multirow{2}{*}{\textbf{Target}} & \textbf{Lag } & \textbf{SHAP }& \textbf{Weight }&\textbf{Ensembles }\\
   & &{\bf (days)} &{\bf Weight} & $\sigma$ & {\bf with edge} \\ 
        \hline
Globe\_T050&Globe\_T050&1&2.41E-01&3.55E-02&5\\
Globe\_FLNTC&Globe\_FLNTC&1&1.73E-01&1.43E-02&5\\
Globe\_AEROD\_v&Globe\_AEROD\_v&1&1.31E-01&7.32E-03&5\\
Globe\_T050&Globe\_T050&6&4.56E-03&3.20E-03&5\\
Globe\_T050&Globe\_T050&36&1.95E-03&2.51E-03&4\\
Globe\_FLNTC&Globe\_FLNTC&6&1.49E-03&7.78E-04&5\\
Globe\_T050&Globe\_T050&11&1.47E-03&1.72E-03&4\\
Globe\_T050&Globe\_T050&41&1.31E-03&2.26E-03&5\\
Globe\_T050&Globe\_T050&16&1.15E-03&1.80E-03&5\\
Globe\_T050&Globe\_T050&21&1.11E-03&6.30E-04&4\\
Globe\_T050&Globe\_T050&26&1.06E-03&9.23E-04&4\\
Globe\_T050&Globe\_T050&31&7.73E-04&6.61E-04&3\\
Globe\_AEROD\_v&Globe\_FLNTC&6&5.62E-04&4.28E-04&5\\
Globe\_AEROD\_v&Globe\_T050&51&5.40E-04&7.35E-04&4\\
Globe\_FLNTC&Globe\_FLNTC&36&5.26E-04&5.65E-04&5\\
Globe\_AEROD\_v&Globe\_T050&46&5.18E-04&7.57E-04&4\\
Globe\_FLNTC&Globe\_FLNTC&56&4.56E-04&3.02E-04&5\\
Globe\_T050&Globe\_T050&46&4.50E-04&5.39E-04&4\\
Globe\_FLNTC&Globe\_FLNTC&31&4.04E-04&2.83E-04&5\\
Globe\_FLNTC&Globe\_AEROD\_v&31&4.00E-04&2.32E-04&4\\
Globe\_FLNTC&Globe\_FLNTC&41&3.96E-04&1.84E-04&5\\
Globe\_FLNTC&Globe\_FLNTC&26&3.90E-04&1.72E-04&5\\
Globe\_AEROD\_v&Globe\_FLNTC&26&3.78E-04&3.58E-04&5\\
Globe\_FLNTC&Globe\_FLNTC&11&3.78E-04&1.93E-04&5\\
Globe\_T050&Globe\_FLNTC&1&3.66E-04&2.29E-04&5\\
Globe\_FLNTC&Globe\_FLNTC&16&3.52E-04&2.42E-04&5\\
Globe\_FLNTC&Globe\_FLNTC&46&3.50E-04&2.14E-04&5\\
Globe\_T050&Globe\_T050&56&3.15E-04&4.94E-04&4\\
Globe\_AEROD\_v&Globe\_FLNTC&11&3.08E-04&1.48E-04&5\\
Globe\_FLNTC&Globe\_FLNTC&21&3.02E-04&4.90E-05&5\\
Globe\_AEROD\_v&Globe\_FLNTC&51&2.90E-04&1.76E-04&5\\
Globe\_AEROD\_v&Globe\_FLNTC&36&2.86E-04&1.05E-04&5\\
Globe\_AEROD\_v&Globe\_FLNTC&31&2.78E-04&2.28E-04&5\\
Globe\_T050&Globe\_FLNTC&31&2.40E-04&2.14E-04&5\\
Globe\_T050&Globe\_FLNTC&26&2.40E-04&1.45E-04&5\\
Globe\_AEROD\_v&Globe\_T050&1&2.33E-04&3.13E-04&4\\
Globe\_AEROD\_v&Globe\_FLNTC&21&2.30E-04&4.90E-05&5\\
Globe\_FLNTC&Globe\_FLNTC&51&2.28E-04&8.70E-05&5\\
Globe\_AEROD\_v&Globe\_FLNTC&1&2.20E-04&8.80E-05&5\\
Globe\_AEROD\_v&Globe\_FLNTC&56&2.08E-04&1.04E-04&5\\
Globe\_T050&Globe\_FLNTC&11&2.02E-04&1.54E-04&5\\
Globe\_T050&Globe\_FLNTC&56&1.98E-04&1.29E-04&5\\
Globe\_T050&Globe\_FLNTC&6&1.94E-04&7.80E-05&5\\
Globe\_AEROD\_v&Globe\_T050&21&1.90E-04&1.60E-04&2\\
Globe\_AEROD\_v&Globe\_FLNTC&41&1.84E-04&1.66E-04&5\\
Globe\_T050&Globe\_FLNTC&16&1.80E-04&1.82E-04&5\\
Globe\_T050&Globe\_FLNTC&21&1.56E-04&7.70E-05&5\\
Globe\_AEROD\_v&Globe\_FLNTC&16&1.48E-04&7.40E-05&5\\
Globe\_FLNTC&Globe\_AEROD\_v&26&1.48E-04&7.70E-05&5\\
Globe\_FLNTC&Globe\_T050&36&1.43E-04&8.20E-05&3\\
Globe\_FLNTC&Globe\_AEROD\_v&41&1.40E-04&1.33E-04&5\\
Globe\_AEROD\_v&Globe\_T050&31&1.37E-04&1.27E-04&3\\
Globe\_AEROD\_v&Globe\_T050&41&1.35E-04&9.50E-05&2\\
Globe\_FLNTC&Globe\_AEROD\_v&46&1.35E-04&1.88E-04&4\\
Globe\_T050&Globe\_AEROD\_v&21&1.35E-04&1.82E-04&4\\
Globe\_T050&Globe\_FLNTC&46&1.34E-04&5.50E-05&5\\
Globe\_T050&Globe\_FLNTC&41&1.16E-04&5.30E-05&5\\
Globe\_AEROD\_v&Globe\_FLNTC&46&1.16E-04&6.30E-05&5\\
Globe\_FLNTC&Globe\_T050&56&1.10E-04&9.40E-05&3\\
Globe\_AEROD\_v&Globe\_T050&36&1.07E-04&9.00E-05&3\\
Globe\_T050&Globe\_FLNTC&51&1.06E-04&7.40E-05&5\\
Globe\_FLNTC&Globe\_T050&21&1.05E-04&8.00E-05&4\\
Globe\_FLNTC&Globe\_AEROD\_v&56&1.03E-04&1.04E-04&3\\
Globe\_AEROD\_v&Globe\_T050&6&1.03E-04&5.90E-05&3\\
Globe\_AEROD\_v&Globe\_AEROD\_v&56&9.20E-05&1.80E-05&4\\
Globe\_FLNTC&Globe\_T050&6&8.80E-05&1.05E-04&4\\
Globe\_AEROD\_v&Globe\_T050&56&8.70E-05&1.23E-04&4\\
Globe\_T050&Globe\_FLNTC&36&8.60E-05&1.40E-05&5\\
Globe\_AEROD\_v&Globe\_AEROD\_v&36&8.30E-05&7.50E-05&4\\
Globe\_FLNTC&Globe\_AEROD\_v&16&8.00E-05&6.10E-05&5\\
Globe\_T050&Globe\_AEROD\_v&1&8.00E-05&2.80E-05&5\\
Globe\_AEROD\_v&Globe\_AEROD\_v&31&8.00E-05&5.70E-05&4\\
Globe\_FLNTC&Globe\_AEROD\_v&11&7.60E-05&9.70E-05&5\\
Globe\_FLNTC&Globe\_AEROD\_v&1&7.40E-05&5.70E-05&5\\
Globe\_FLNTC&Globe\_AEROD\_v&21&7.20E-05&7.90E-05&5\\
Globe\_AEROD\_v&Globe\_AEROD\_v&21&7.00E-05&4.70E-05&5\\
Globe\_AEROD\_v&Globe\_AEROD\_v&51&7.00E-05&3.20E-05&5\\
Globe\_AEROD\_v&Globe\_AEROD\_v&46&7.00E-05&3.70E-05&4\\
Globe\_T050&Globe\_AEROD\_v&46&6.80E-05&1.11E-04&5\\
Globe\_FLNTC&Globe\_AEROD\_v&6&6.80E-05&4.40E-05&5\\
Globe\_T050&Globe\_T050&51&6.70E-05&5.40E-05&3\\
Globe\_T050&Globe\_AEROD\_v&51&6.00E-05&2.80E-05&5\\
Globe\_T050&Globe\_AEROD\_v&6&5.70E-05&8.00E-06&4\\
Globe\_FLNTC&Globe\_T050&26&5.70E-05&4.10E-05&3\\
Globe\_T050&Globe\_AEROD\_v&31&5.60E-05&6.10E-05&5\\
Globe\_AEROD\_v&Globe\_AEROD\_v&11&5.40E-05&2.70E-05&5\\
Globe\_T050&Globe\_AEROD\_v&11&5.30E-05&5.40E-05&3\\
Globe\_FLNTC&Globe\_AEROD\_v&51&5.20E-05&2.60E-05&5\\
Globe\_AEROD\_v&Globe\_AEROD\_v&41&5.00E-05&9.00E-06&5\\
Globe\_AEROD\_v&Globe\_T050&26&5.00E-05&3.70E-05&5\\
Globe\_AEROD\_v&Globe\_AEROD\_v&16&4.40E-05&3.40E-05&5\\
Globe\_T050&Globe\_AEROD\_v&36&4.30E-05&3.70E-05&4\\
Globe\_AEROD\_v&Globe\_AEROD\_v&6&4.00E-05&1.60E-05&4\\
Globe\_T050&Globe\_AEROD\_v&41&3.80E-05&1.70E-05&5\\
Globe\_FLNTC&Globe\_AEROD\_v&36&3.80E-05&1.50E-05&4\\
Globe\_FLNTC&Globe\_T050&51&3.70E-05&3.80E-05&3\\
Globe\_AEROD\_v&Globe\_AEROD\_v&26&3.60E-05&1.90E-05&5\\
Globe\_FLNTC&Globe\_T050&11&3.50E-05&2.50E-05&2\\
Globe\_AEROD\_v&Globe\_T050&11&3.20E-05&2.70E-05&5\\
Globe\_FLNTC&Globe\_T050&16&3.20E-05&1.70E-05&5\\
Globe\_T050&Globe\_AEROD\_v&56&3.00E-05&1.90E-05&5\\
Globe\_T050&Globe\_AEROD\_v&16&3.00E-05&1.40E-05&3\\
Globe\_FLNTC&Globe\_T050&31&2.60E-05&1.90E-05&5\\
Globe\_FLNTC&Globe\_T050&41&2.30E-05&5.00E-06&3\\
Globe\_AEROD\_v&Globe\_T050&16&2.30E-05&9.00E-06&3\\
Globe\_FLNTC&Globe\_T050&1&1.80E-05&8.00E-06&4\\
Globe\_T050&Globe\_AEROD\_v&26&1.67E-05&9.43E-06&2\\
Globe\_FLNTC&Globe\_T050&46&1.00E-05&0.00E+00&2\\
\hline
\end{longtblr}

\subsection*{A.2.  Global Surface}
\begin{longtblr}[
  caption = {Mount Pinatubo exemplar: unpruned pathway edge weights and their standard deviations for the surface cooling pathway obtained using globally-averaged data windowed to 750 days.},
  label = {tab:app_global_surf},
]{
  colspec = {llcccc},
  width=\textwidth,rowsep=0pt,
  cells={font=\small},
  rowhead = 2,
} 

    \hline \hline
        \textbf{Source} & \textbf{Target} & \textbf{Lag(days)}&\textbf{SHAP Weight} & \textbf{Weight $\sigma$}& \textbf{Ensembles with edge} \\
        \hline
Globe\_TREFHT&Globe\_TREFHT&1&2.07E-01&3.44E-02&5\\
Globe\_AEROD\_v&Globe\_AEROD\_v&1&1.31E-01&7.34E-03&5\\
Globe\_FSDSC&Globe\_FSDSC&1&1.29E-01&8.63E-03&5\\
Globe\_TREFHT&Globe\_TREFHT&6&1.04E-03&7.82E-04&5\\
Globe\_AEROD\_v&Globe\_FSDSC&1&1.03E-03&6.52E-04&5\\
Globe\_FSDSC&Globe\_TREFHT&51&5.52E-04&3.81E-04&5\\
Globe\_TREFHT&Globe\_TREFHT&26&5.24E-04&3.70E-04&5\\
Globe\_TREFHT&Globe\_TREFHT&46&5.14E-04&3.09E-04&5\\
Globe\_TREFHT&Globe\_TREFHT&11&4.96E-04&1.44E-04&5\\
Globe\_FSDSC&Globe\_TREFHT&56&4.94E-04&4.18E-04&5\\
Globe\_TREFHT&Globe\_TREFHT&31&4.74E-04&4.16E-04&5\\
Globe\_TREFHT&Globe\_TREFHT&51&4.58E-04&3.37E-04&5\\
Globe\_TREFHT&Globe\_TREFHT&36&4.06E-04&1.66E-04&5\\
Globe\_AEROD\_v&Globe\_TREFHT&41&3.64E-04&3.67E-04&5\\
Globe\_TREFHT&Globe\_TREFHT&41&3.62E-04&2.16E-04&5\\
Globe\_TREFHT&Globe\_TREFHT&21&3.30E-04&1.98E-04&5\\
Globe\_TREFHT&Globe\_TREFHT&16&3.08E-04&1.51E-04&5\\
Globe\_FSDSC&Globe\_TREFHT&36&2.90E-04&1.01E-04&5\\
Globe\_FSDSC&Globe\_TREFHT&46&2.80E-04&1.95E-04&5\\
Globe\_FSDSC&Globe\_TREFHT&1&2.66E-04&1.22E-04&5\\
Globe\_AEROD\_v&Globe\_TREFHT&31&2.52E-04&2.26E-04&5\\
Globe\_TREFHT&Globe\_TREFHT&56&2.38E-04&5.80E-05&5\\
Globe\_AEROD\_v&Globe\_TREFHT&46&2.38E-04&1.78E-04&5\\
Globe\_AEROD\_v&Globe\_TREFHT&6&2.32E-04&4.30E-05&5\\
Globe\_FSDSC&Globe\_AEROD\_v&21&2.27E-04&7.00E-05&4\\
Globe\_AEROD\_v&Globe\_TREFHT&56&2.24E-04&8.20E-05&5\\
Globe\_TREFHT&Globe\_FSDSC&51&2.20E-04&2.71E-04&5\\
Globe\_AEROD\_v&Globe\_TREFHT&16&2.16E-04&1.72E-04&5\\
Globe\_AEROD\_v&Globe\_TREFHT&36&2.16E-04&1.10E-04&5\\
Globe\_FSDSC&Globe\_FSDSC&21&2.12E-04&8.30E-05&4\\
Globe\_FSDSC&Globe\_TREFHT&16&1.98E-04&7.90E-05&5\\
Globe\_FSDSC&Globe\_AEROD\_v&56&1.95E-04&2.14E-04&4\\
Globe\_FSDSC&Globe\_TREFHT&21&1.94E-04&7.70E-05&5\\
Globe\_FSDSC&Globe\_TREFHT&11&1.90E-04&1.26E-04&5\\
Globe\_AEROD\_v&Globe\_TREFHT&11&1.82E-04&1.46E-04&5\\
Globe\_AEROD\_v&Globe\_TREFHT&1&1.80E-04&6.40E-05&5\\
Globe\_FSDSC&Globe\_TREFHT&6&1.76E-04&1.14E-04&5\\
Globe\_AEROD\_v&Globe\_TREFHT&21&1.74E-04&8.70E-05&5\\
Globe\_FSDSC&Globe\_TREFHT&26&1.74E-04&1.22E-04&5\\
Globe\_TREFHT&Globe\_FSDSC&1&1.64E-04&9.50E-05&5\\
Globe\_AEROD\_v&Globe\_TREFHT&51&1.60E-04&8.90E-05&5\\
Globe\_AEROD\_v&Globe\_TREFHT&26&1.56E-04&8.30E-05&5\\
Globe\_FSDSC&Globe\_TREFHT&41&1.50E-04&8.00E-05&5\\
Globe\_FSDSC&Globe\_AEROD\_v&1&1.48E-04&1.79E-04&5\\
Globe\_FSDSC&Globe\_AEROD\_v&46&1.34E-04&2.18E-04&5\\
Globe\_FSDSC&Globe\_FSDSC&26&1.22E-04&7.00E-05&4\\
Globe\_FSDSC&Globe\_FSDSC&6&1.22E-04&8.80E-05&5\\
Globe\_TREFHT&Globe\_FSDSC&41&1.12E-04&8.50E-05&5\\
Globe\_TREFHT&Globe\_FSDSC&21&1.10E-04&6.00E-05&4\\
Globe\_AEROD\_v&Globe\_FSDSC&41&1.10E-04&1.12E-04&5\\
Globe\_TREFHT&Globe\_FSDSC&36&1.08E-04&1.21E-04&5\\
Globe\_AEROD\_v&Globe\_FSDSC&16&1.00E-04&5.20E-05&4\\
Globe\_TREFHT&Globe\_FSDSC&46&9.60E-05&7.60E-05&5\\
Globe\_FSDSC&Globe\_TREFHT&31&9.60E-05&3.40E-05&5\\
Globe\_FSDSC&Globe\_AEROD\_v&6&9.40E-05&5.60E-05&5\\
Globe\_FSDSC&Globe\_AEROD\_v&51&9.00E-05&8.50E-05&3\\
Globe\_AEROD\_v&Globe\_AEROD\_v&21&9.00E-05&7.90E-05&5\\
Globe\_AEROD\_v&Globe\_AEROD\_v&56&9.00E-05&6.30E-05&5\\
Globe\_AEROD\_v&Globe\_FSDSC&11&9.00E-05&6.00E-05&5\\
Globe\_FSDSC&Globe\_FSDSC&56&8.80E-05&8.40E-05&5\\
Globe\_AEROD\_v&Globe\_AEROD\_v&31&8.80E-05&1.80E-05&5\\
Globe\_AEROD\_v&Globe\_FSDSC&31&8.40E-05&6.70E-05&5\\
Globe\_TREFHT&Globe\_AEROD\_v&31&8.40E-05&8.30E-05&5\\
Globe\_FSDSC&Globe\_FSDSC&16&8.00E-05&5.40E-05&5\\
Globe\_TREFHT&Globe\_FSDSC&6&8.00E-05&3.00E-05&5\\
Globe\_TREFHT&Globe\_FSDSC&56&8.00E-05&3.60E-05&5\\
Globe\_FSDSC&Globe\_FSDSC&11&7.40E-05&3.40E-05&5\\
Globe\_TREFHT&Globe\_AEROD\_v&6&7.30E-05&6.80E-05&4\\
Globe\_FSDSC&Globe\_FSDSC&31&7.20E-05&6.00E-05&5\\
Globe\_TREFHT&Globe\_FSDSC&26&7.20E-05&2.30E-05&5\\
Globe\_AEROD\_v&Globe\_FSDSC&26&7.00E-05&5.10E-05&5\\
Globe\_TREFHT&Globe\_AEROD\_v&46&7.00E-05&5.90E-05&5\\
Globe\_TREFHT&Globe\_AEROD\_v&26&7.00E-05&5.40E-05&4\\
Globe\_AEROD\_v&Globe\_FSDSC&6&6.80E-05&4.10E-05&5\\
Globe\_TREFHT&Globe\_FSDSC&31&6.60E-05&5.30E-05&5\\
Globe\_FSDSC&Globe\_AEROD\_v&16&6.60E-05&3.20E-05&5\\
Globe\_FSDSC&Globe\_AEROD\_v&26&6.50E-05&7.80E-05&4\\
Globe\_TREFHT&Globe\_AEROD\_v&51&6.40E-05&6.60E-05&5\\
Globe\_AEROD\_v&Globe\_FSDSC&56&6.40E-05&4.00E-05&5\\
Globe\_FSDSC&Globe\_FSDSC&41&6.00E-05&3.00E-05&5\\
Globe\_TREFHT&Globe\_AEROD\_v&16&6.00E-05&4.10E-05&5\\
Globe\_TREFHT&Globe\_FSDSC&16&5.80E-05&5.10E-05&5\\
Globe\_TREFHT&Globe\_AEROD\_v&36&5.80E-05&3.10E-05&5\\
Globe\_AEROD\_v&Globe\_FSDSC&36&5.80E-05&3.30E-05&5\\
Globe\_FSDSC&Globe\_AEROD\_v&41&5.60E-05&3.90E-05&5\\
Globe\_AEROD\_v&Globe\_AEROD\_v&41&5.60E-05&2.90E-05&5\\
Globe\_AEROD\_v&Globe\_AEROD\_v&36&5.50E-05&2.70E-05&4\\
Globe\_AEROD\_v&Globe\_FSDSC&46&5.40E-05&3.40E-05&5\\
Globe\_TREFHT&Globe\_FSDSC&11&5.20E-05&2.60E-05&5\\
Globe\_TREFHT&Globe\_AEROD\_v&21&5.20E-05&6.00E-05&5\\
Globe\_TREFHT&Globe\_AEROD\_v&11&5.00E-05&4.60E-05&5\\
Globe\_AEROD\_v&Globe\_FSDSC&51&5.00E-05&1.60E-05&4\\
Globe\_FSDSC&Globe\_FSDSC&36&5.00E-05&3.70E-05&3\\
Globe\_FSDSC&Globe\_FSDSC&51&5.00E-05&3.20E-05&4\\
Globe\_TREFHT&Globe\_AEROD\_v&41&4.80E-05&2.70E-05&5\\
Globe\_AEROD\_v&Globe\_FSDSC&21&4.80E-05&3.20E-05&5\\
Globe\_AEROD\_v&Globe\_AEROD\_v&16&4.50E-05&4.40E-05&4\\
Globe\_AEROD\_v&Globe\_AEROD\_v&26&4.50E-05&1.50E-05&4\\
Globe\_AEROD\_v&Globe\_AEROD\_v&6&4.30E-05&3.70E-05&4\\
Globe\_FSDSC&Globe\_FSDSC&46&4.00E-05&1.90E-05&4\\
Globe\_TREFHT&Globe\_AEROD\_v&56&4.00E-05&4.60E-05&5\\
Globe\_FSDSC&Globe\_AEROD\_v&11&3.80E-05&2.70E-05&5\\
Globe\_TREFHT&Globe\_AEROD\_v&1&3.60E-05&1.00E-05&5\\
Globe\_FSDSC&Globe\_AEROD\_v&36&3.50E-05&1.10E-05&4\\
Globe\_AEROD\_v&Globe\_AEROD\_v&11&3.20E-05&1.00E-05&5\\
Globe\_AEROD\_v&Globe\_AEROD\_v&51&3.20E-05&2.00E-05&5\\
Globe\_AEROD\_v&Globe\_AEROD\_v&46&3.00E-05&2.10E-05&5\\
Globe\_FSDSC&Globe\_AEROD\_v&31&2.80E-05&1.60E-05&5\\
\hline
\end{longtblr}

\subsection*{A.3.  Regional Stratosphere}
\begin{longtblr}[
  caption = {Mount Pinatubo exemplar: unpruned pathway edge weights and their standard deviations for the stratospheric warming pathway obtained using zonally-averaged data windowed to 750 days.},
  label = {tab:app_tropics_strat},
]{
  colspec = {llcccc},
  width=\textwidth,rowsep=0pt,
  cells={font=\small},
  rowhead = 2,
} 

    \hline \hline
        \multirow{2}{*}{\textbf{Source}} & \multirow{2}{*}{\textbf{Target}} & \textbf{Lag } & \textbf{SHAP }& \textbf{Weight }&\textbf{Ensembles }\\
   & &{\bf (days)} &{\bf Weight} & $\sigma$ & {\bf with edge} \\ 
        \hline
SubtropN\_T050&SubtropN\_T050&1&1.91E-01&4.21E-02&5\\
Tropical\_T050&Tropical\_T050&1&1.91E-01&5.20E-02&5\\
SubtropN\_FLNTC&SubtropN\_FLNTC&1&1.89E-01&2.58E-02&5\\
Tropical\_AEROD\_v&Tropical\_AEROD\_v&1&1.57E-01&2.04E-02&5\\
SubtropN\_AEROD\_v&SubtropN\_AEROD\_v&1&1.39E-01&2.22E-02&5\\
Tropical\_FLNTC&Tropical\_FLNTC&1&1.17E-01&1.09E-02&5\\
Tropical\_AEROD\_v&Tropical\_T050&1&1.39E-03&0.00E+00&1\\
Tropical\_T050&Tropical\_AEROD\_v&6&1.25E-03&1.23E-03&2\\
Tropical\_FLNTC&SubtropN\_FLNTC&1&9.52E-04&6.53E-04&5\\
Tropical\_T050&SubtropN\_T050&21&9.13E-04&8.15E-04&3\\
SubtropN\_FLNTC&SubtropN\_FLNTC&46&9.06E-04&6.95E-04&5\\
SubtropN\_FLNTC&SubtropN\_FLNTC&21&8.42E-04&5.14E-04&4\\
Tropical\_T050&Tropical\_AEROD\_v&21&7.90E-04&1.09E-03&3\\
Tropical\_T050&SubtropN\_T050&46&7.08E-04&7.49E-04&5\\
SubtropN\_AEROD\_v&SubtropN\_FLNTC&1&6.90E-04&2.82E-04&5\\
SubtropN\_FLNTC&SubtropN\_FLNTC&6&6.74E-04&3.91E-04&5\\
Tropical\_AEROD\_v&SubtropN\_AEROD\_v&6&6.20E-04&5.25E-04&5\\
Tropical\_T050&SubtropN\_FLNTC&31&6.02E-04&7.05E-04&5\\
Tropical\_T050&SubtropN\_FLNTC&51&6.00E-04&5.70E-04&5\\
SubtropN\_AEROD\_v&SubtropN\_FLNTC&41&5.66E-04&3.42E-04&5\\
SubtropN\_AEROD\_v&SubtropN\_FLNTC&6&5.54E-04&2.64E-04&5\\
Tropical\_T050&SubtropN\_T050&11&5.54E-04&9.48E-04&5\\
SubtropN\_FLNTC&SubtropN\_FLNTC&51&5.48E-04&1.64E-04&5\\
Tropical\_AEROD\_v&SubtropN\_FLNTC&46&5.38E-04&4.17E-04&5\\
SubtropN\_AEROD\_v&SubtropN\_FLNTC&21&5.34E-04&3.22E-04&5\\
SubtropN\_FLNTC&SubtropN\_FLNTC&16&5.08E-04&2.06E-04&5\\
Tropical\_T050&SubtropN\_FLNTC&46&5.06E-04&4.72E-04&5\\
Tropical\_FLNTC&Tropical\_FLNTC&6&5.04E-04&2.89E-04&5\\
SubtropN\_T050&Tropical\_AEROD\_v&21&4.95E-04&4.55E-04&2\\
SubtropN\_FLNTC&SubtropN\_FLNTC&56&4.84E-04&3.77E-04&5\\
SubtropN\_FLNTC&SubtropN\_FLNTC&26&4.82E-04&1.80E-04&5\\
SubtropN\_T050&SubtropN\_T050&56&4.80E-04&6.39E-04&5\\
Tropical\_FLNTC&SubtropN\_FLNTC&26&4.70E-04&3.83E-04&5\\
SubtropN\_T050&SubtropN\_FLNTC&46&4.46E-04&2.79E-04&5\\
Tropical\_AEROD\_v&Tropical\_FLNTC&6&4.42E-04&2.49E-04&5\\
Tropical\_AEROD\_v&SubtropN\_FLNTC&21&4.38E-04&4.81E-04&5\\
Tropical\_AEROD\_v&SubtropN\_FLNTC&26&4.35E-04&2.07E-04&4\\
Tropical\_FLNTC&SubtropN\_FLNTC&51&4.34E-04&3.76E-04&5\\
SubtropN\_AEROD\_v&SubtropN\_FLNTC&16&4.34E-04&3.77E-04&5\\
Tropical\_T050&SubtropN\_T050&6&4.27E-04&5.91E-04&4\\
Tropical\_FLNTC&SubtropN\_FLNTC&56&4.16E-04&3.21E-04&5\\
Tropical\_AEROD\_v&SubtropN\_FLNTC&36&4.04E-04&4.59E-04&5\\
Tropical\_FLNTC&SubtropN\_FLNTC&16&4.04E-04&4.80E-04&5\\
Tropical\_AEROD\_v&SubtropN\_FLNTC&6&3.90E-04&3.18E-04&5\\
SubtropN\_AEROD\_v&SubtropN\_FLNTC&31&3.84E-04&4.41E-04&5\\
Tropical\_T050&Tropical\_AEROD\_v&41&3.83E-04&6.05E-04&4\\
SubtropN\_AEROD\_v&SubtropN\_FLNTC&11&3.80E-04&2.05E-04&5\\
Tropical\_AEROD\_v&SubtropN\_FLNTC&16&3.78E-04&2.52E-04&5\\
Tropical\_FLNTC&SubtropN\_FLNTC&31&3.78E-04&2.12E-04&5\\
SubtropN\_FLNTC&SubtropN\_FLNTC&36&3.72E-04&1.54E-04&5\\
Tropical\_FLNTC&SubtropN\_FLNTC&11&3.68E-04&1.49E-04&5\\
SubtropN\_AEROD\_v&SubtropN\_FLNTC&46&3.62E-04&2.53E-04&5\\
SubtropN\_AEROD\_v&SubtropN\_FLNTC&36&3.56E-04&1.42E-04&5\\
Tropical\_T050&SubtropN\_T050&36&3.54E-04&2.63E-04&5\\
SubtropN\_T050&SubtropN\_FLNTC&1&3.52E-04&4.08E-04&5\\
Tropical\_FLNTC&SubtropN\_AEROD\_v&1&3.52E-04&3.28E-04&5\\
SubtropN\_FLNTC&SubtropN\_FLNTC&11&3.50E-04&2.95E-04&5\\
SubtropN\_AEROD\_v&SubtropN\_FLNTC&51&3.50E-04&1.75E-04&5\\
Tropical\_FLNTC&Tropical\_FLNTC&16&3.48E-04&2.85E-04&5\\
SubtropN\_AEROD\_v&SubtropN\_AEROD\_v&46&3.42E-04&2.72E-04&5\\
SubtropN\_FLNTC&SubtropN\_FLNTC&41&3.42E-04&1.27E-04&5\\
Tropical\_FLNTC&SubtropN\_FLNTC&6&3.42E-04&2.00E-04&5\\
SubtropN\_AEROD\_v&SubtropN\_AEROD\_v&6&3.34E-04&1.82E-04&5\\
SubtropN\_T050&SubtropN\_FLNTC&41&3.34E-04&2.72E-04&5\\
SubtropN\_AEROD\_v&SubtropN\_AEROD\_v&11&3.32E-04&1.89E-04&5\\
Tropical\_AEROD\_v&SubtropN\_FLNTC&31&3.26E-04&1.82E-04&5\\
Tropical\_FLNTC&SubtropN\_AEROD\_v&11&3.22E-04&1.59E-04&5\\
Tropical\_AEROD\_v&SubtropN\_AEROD\_v&21&3.20E-04&1.32E-04&5\\
SubtropN\_AEROD\_v&SubtropN\_AEROD\_v&16&3.18E-04&1.35E-04&5\\
Tropical\_T050&SubtropN\_T050&51&3.10E-04&1.86E-04&4\\
Tropical\_T050&SubtropN\_FLNTC&36&3.08E-04&1.80E-04&5\\
SubtropN\_T050&SubtropN\_AEROD\_v&46&3.06E-04&2.95E-04&5\\
Tropical\_AEROD\_v&SubtropN\_AEROD\_v&36&3.00E-04&2.96E-04&5\\
SubtropN\_AEROD\_v&SubtropN\_FLNTC&26&2.94E-04&1.36E-04&5\\
Tropical\_FLNTC&SubtropN\_AEROD\_v&16&2.92E-04&2.63E-04&5\\
SubtropN\_FLNTC&SubtropN\_FLNTC&31&2.90E-04&1.72E-04&5\\
Tropical\_FLNTC&Tropical\_FLNTC&11&2.90E-04&1.80E-04&5\\
Tropical\_FLNTC&SubtropN\_FLNTC&41&2.84E-04&1.58E-04&5\\
Tropical\_FLNTC&Tropical\_FLNTC&21&2.82E-04&1.02E-04&5\\
Tropical\_AEROD\_v&SubtropN\_FLNTC&11&2.76E-04&1.03E-04&5\\
Tropical\_AEROD\_v&SubtropN\_FLNTC&56&2.76E-04&2.24E-04&5\\
Tropical\_AEROD\_v&SubtropN\_AEROD\_v&11&2.74E-04&1.55E-04&5\\
SubtropN\_FLNTC&SubtropN\_AEROD\_v&1&2.72E-04&1.02E-04&5\\
SubtropN\_AEROD\_v&SubtropN\_AEROD\_v&36&2.68E-04&1.24E-04&5\\
SubtropN\_FLNTC&Tropical\_FLNTC&1&2.64E-04&1.43E-04&5\\
SubtropN\_FLNTC&Tropical\_FLNTC&36&2.64E-04&1.62E-04&5\\
Tropical\_AEROD\_v&Tropical\_FLNTC&26&2.62E-04&1.51E-04&5\\
SubtropN\_FLNTC&Tropical\_FLNTC&11&2.58E-04&1.56E-04&5\\
Tropical\_T050&SubtropN\_T050&41&2.55E-04&2.86E-04&4\\
SubtropN\_T050&SubtropN\_FLNTC&51&2.54E-04&1.39E-04&5\\
Tropical\_FLNTC&SubtropN\_FLNTC&46&2.52E-04&1.54E-04&5\\
Tropical\_T050&SubtropN\_FLNTC&21&2.46E-04&1.40E-04&5\\
Tropical\_AEROD\_v&SubtropN\_AEROD\_v&41&2.44E-04&1.82E-04&5\\
Tropical\_AEROD\_v&SubtropN\_AEROD\_v&31&2.44E-04&5.60E-05&5\\
Tropical\_AEROD\_v&SubtropN\_FLNTC&41&2.42E-04&1.67E-04&5\\
Tropical\_T050&SubtropN\_FLNTC&56&2.42E-04&2.05E-04&5\\
Tropical\_FLNTC&SubtropN\_FLNTC&21&2.36E-04&1.30E-04&5\\
Tropical\_FLNTC&SubtropN\_AEROD\_v&51&2.36E-04&9.20E-05&5\\
SubtropN\_T050&SubtropN\_AEROD\_v&1&2.34E-04&2.69E-04&5\\
SubtropN\_AEROD\_v&Tropical\_FLNTC&6&2.32E-04&1.60E-04&5\\
SubtropN\_T050&SubtropN\_AEROD\_v&6&2.32E-04&2.86E-04&5\\
Tropical\_FLNTC&SubtropN\_AEROD\_v&46&2.32E-04&1.00E-04&5\\
SubtropN\_AEROD\_v&SubtropN\_AEROD\_v&26&2.30E-04&9.50E-05&5\\
Tropical\_FLNTC&SubtropN\_AEROD\_v&36&2.30E-04&2.07E-04&5\\
Tropical\_T050&SubtropN\_FLNTC&1&2.28E-04&2.71E-04&5\\
Tropical\_T050&SubtropN\_AEROD\_v&16&2.26E-04&1.95E-04&5\\
SubtropN\_T050&SubtropN\_FLNTC&56&2.24E-04&7.70E-05&5\\
Tropical\_AEROD\_v&Tropical\_FLNTC&11&2.22E-04&1.20E-04&5\\
Tropical\_FLNTC&SubtropN\_FLNTC&36&2.18E-04&1.93E-04&5\\
SubtropN\_AEROD\_v&SubtropN\_FLNTC&56&2.18E-04&1.19E-04&5\\
SubtropN\_FLNTC&Tropical\_FLNTC&51&2.18E-04&1.37E-04&5\\
SubtropN\_FLNTC&Tropical\_FLNTC&56&2.16E-04&1.17E-04&5\\
Tropical\_T050&SubtropN\_AEROD\_v&51&2.12E-04&2.08E-04&5\\
SubtropN\_FLNTC&SubtropN\_AEROD\_v&21&2.08E-04&1.32E-04&5\\
SubtropN\_T050&SubtropN\_AEROD\_v&16&2.06E-04&2.18E-04&5\\
Tropical\_T050&SubtropN\_AEROD\_v&56&2.06E-04&2.10E-04&5\\
SubtropN\_T050&Tropical\_T050&56&2.05E-04&1.85E-04&2\\
Tropical\_FLNTC&SubtropN\_AEROD\_v&41&2.04E-04&1.22E-04&5\\
SubtropN\_FLNTC&SubtropN\_AEROD\_v&41&2.04E-04&8.40E-05&5\\
SubtropN\_FLNTC&SubtropN\_AEROD\_v&31&2.02E-04&1.99E-04&5\\
SubtropN\_FLNTC&SubtropN\_AEROD\_v&51&2.00E-04&1.43E-04&5\\
SubtropN\_FLNTC&Tropical\_FLNTC&46&2.00E-04&1.08E-04&5\\
SubtropN\_AEROD\_v&Tropical\_FLNTC&1&1.96E-04&1.03E-04&5\\
SubtropN\_AEROD\_v&Tropical\_FLNTC&31&1.96E-04&1.24E-04&5\\
SubtropN\_FLNTC&Tropical\_FLNTC&6&1.94E-04&4.40E-05&5\\
SubtropN\_AEROD\_v&Tropical\_FLNTC&56&1.94E-04&7.80E-05&5\\
Tropical\_FLNTC&Tropical\_FLNTC&26&1.94E-04&7.70E-05&5\\
SubtropN\_T050&SubtropN\_FLNTC&6&1.92E-04&1.38E-04&5\\
Tropical\_T050&Tropical\_AEROD\_v&16&1.90E-04&2.48E-04&3\\
Tropical\_AEROD\_v&SubtropN\_AEROD\_v&16&1.86E-04&1.29E-04&5\\
Tropical\_AEROD\_v&SubtropN\_AEROD\_v&51&1.86E-04&1.52E-04&5\\
SubtropN\_AEROD\_v&SubtropN\_AEROD\_v&51&1.84E-04&7.70E-05&5\\
Tropical\_FLNTC&Tropical\_FLNTC&51&1.82E-04&1.41E-04&5\\
SubtropN\_AEROD\_v&SubtropN\_T050&31&1.80E-04&1.84E-04&3\\
Tropical\_AEROD\_v&SubtropN\_AEROD\_v&26&1.80E-04&1.00E-04&5\\
Tropical\_AEROD\_v&SubtropN\_T050&31&1.78E-04&1.28E-04&5\\
SubtropN\_AEROD\_v&SubtropN\_AEROD\_v&21&1.78E-04&6.60E-05&5\\
Tropical\_FLNTC&Tropical\_FLNTC&46&1.76E-04&1.04E-04&5\\
Tropical\_AEROD\_v&Tropical\_FLNTC&16&1.76E-04&8.80E-05&5\\
SubtropN\_AEROD\_v&Tropical\_FLNTC&26&1.76E-04&1.47E-04&5\\
SubtropN\_FLNTC&Tropical\_AEROD\_v&16&1.75E-04&1.55E-04&2\\
Tropical\_T050&SubtropN\_FLNTC&6&1.72E-04&1.09E-04&5\\
Tropical\_T050&Tropical\_FLNTC&41&1.70E-04&1.53E-04&5\\
SubtropN\_AEROD\_v&Tropical\_FLNTC&51&1.70E-04&1.37E-04&5\\
SubtropN\_AEROD\_v&Tropical\_FLNTC&16&1.70E-04&1.19E-04&5\\
Tropical\_T050&Tropical\_FLNTC&21&1.70E-04&2.16E-04&5\\
SubtropN\_FLNTC&SubtropN\_AEROD\_v&56&1.68E-04&1.49E-04&5\\
Tropical\_T050&SubtropN\_AEROD\_v&11&1.68E-04&1.22E-04&5\\
SubtropN\_FLNTC&Tropical\_FLNTC&21&1.66E-04&1.03E-04&5\\
Tropical\_AEROD\_v&SubtropN\_AEROD\_v&46&1.66E-04&5.80E-05&5\\
Tropical\_FLNTC&SubtropN\_AEROD\_v&6&1.66E-04&7.70E-05&5\\
Tropical\_FLNTC&Tropical\_FLNTC&31&1.66E-04&6.90E-05&5\\
SubtropN\_AEROD\_v&SubtropN\_AEROD\_v&41&1.64E-04&1.09E-04&5\\
SubtropN\_FLNTC&Tropical\_FLNTC&31&1.64E-04&8.80E-05&5\\
SubtropN\_T050&SubtropN\_FLNTC&21&1.64E-04&5.90E-05&5\\
SubtropN\_AEROD\_v&SubtropN\_AEROD\_v&31&1.62E-04&5.20E-05&5\\
SubtropN\_T050&SubtropN\_AEROD\_v&21&1.62E-04&1.44E-04&5\\
SubtropN\_T050&SubtropN\_FLNTC&36&1.62E-04&1.00E-04&5\\
SubtropN\_AEROD\_v&Tropical\_T050&1&1.60E-04&0.00E+00&1\\
Tropical\_AEROD\_v&SubtropN\_FLNTC&1&1.60E-04&1.69E-04&5\\
SubtropN\_T050&SubtropN\_FLNTC&31&1.58E-04&1.02E-04&5\\
Tropical\_AEROD\_v&SubtropN\_AEROD\_v&56&1.58E-04&5.60E-05&5\\
SubtropN\_T050&SubtropN\_FLNTC&11&1.58E-04&2.20E-05&4\\
SubtropN\_T050&Tropical\_FLNTC&36&1.56E-04&1.46E-04&5\\
Tropical\_FLNTC&Tropical\_FLNTC&56&1.56E-04&1.02E-04&5\\
SubtropN\_T050&SubtropN\_FLNTC&26&1.56E-04&1.39E-04&5\\
Tropical\_AEROD\_v&Tropical\_FLNTC&56&1.54E-04&8.10E-05&5\\
Tropical\_AEROD\_v&SubtropN\_FLNTC&51&1.54E-04&1.20E-04&5\\
SubtropN\_T050&SubtropN\_AEROD\_v&36&1.54E-04&9.50E-05&5\\
SubtropN\_T050&Tropical\_T050&11&1.53E-04&1.62E-04&3\\
Tropical\_AEROD\_v&SubtropN\_T050&46&1.53E-04&1.07E-04&4\\
SubtropN\_FLNTC&Tropical\_FLNTC&16&1.50E-04&7.70E-05&5\\
Tropical\_T050&Tropical\_T050&56&1.50E-04&1.93E-04&4\\
Tropical\_T050&Tropical\_FLNTC&11&1.47E-04&1.59E-04&3\\
Tropical\_AEROD\_v&Tropical\_FLNTC&31&1.46E-04&6.60E-05&5\\
SubtropN\_AEROD\_v&Tropical\_FLNTC&36&1.46E-04&1.09E-04&5\\
SubtropN\_T050&Tropical\_FLNTC&46&1.42E-04&5.70E-05&5\\
SubtropN\_AEROD\_v&Tropical\_FLNTC&41&1.40E-04&6.10E-05&5\\
SubtropN\_T050&SubtropN\_AEROD\_v&51&1.40E-04&9.40E-05&5\\
Tropical\_T050&Tropical\_T050&36&1.40E-04&1.20E-04&2\\
SubtropN\_T050&SubtropN\_T050&6&1.40E-04&1.47E-04&4\\
SubtropN\_FLNTC&SubtropN\_AEROD\_v&36&1.38E-04&3.90E-05&5\\
SubtropN\_AEROD\_v&SubtropN\_AEROD\_v&56&1.38E-04&9.70E-05&5\\
Tropical\_FLNTC&SubtropN\_AEROD\_v&31&1.38E-04&3.50E-05&5\\
SubtropN\_FLNTC&SubtropN\_AEROD\_v&26&1.36E-04&1.19E-04&5\\
Tropical\_T050&SubtropN\_FLNTC&11&1.36E-04&6.60E-05&5\\
Tropical\_T050&SubtropN\_FLNTC&41&1.36E-04&7.30E-05&5\\
Tropical\_AEROD\_v&SubtropN\_T050&16&1.35E-04&7.20E-05&4\\
Tropical\_FLNTC&SubtropN\_AEROD\_v&56&1.34E-04&7.60E-05&5\\
Tropical\_FLNTC&SubtropN\_AEROD\_v&21&1.34E-04&8.20E-05&5\\
Tropical\_AEROD\_v&SubtropN\_AEROD\_v&1&1.34E-04&6.30E-05&5\\
Tropical\_FLNTC&SubtropN\_T050&36&1.33E-04&1.84E-04&4\\
Tropical\_FLNTC&SubtropN\_T050&41&1.32E-04&1.17E-04&5\\
SubtropN\_FLNTC&Tropical\_AEROD\_v&56&1.30E-04&3.00E-05&2\\
Tropical\_T050&Tropical\_FLNTC&36&1.30E-04&1.02E-04&5\\
Tropical\_FLNTC&Tropical\_FLNTC&41&1.30E-04&6.80E-05&5\\
Tropical\_FLNTC&Tropical\_AEROD\_v&1&1.28E-04&2.11E-04&5\\
SubtropN\_FLNTC&SubtropN\_AEROD\_v&6&1.28E-04&5.20E-05&5\\
SubtropN\_FLNTC&Tropical\_AEROD\_v&26&1.28E-04&1.98E-04&4\\
SubtropN\_T050&SubtropN\_AEROD\_v&11&1.24E-04&6.10E-05&5\\
Tropical\_FLNTC&SubtropN\_T050&16&1.20E-04&7.10E-05&5\\
Tropical\_T050&SubtropN\_AEROD\_v&46&1.20E-04&7.80E-05&5\\
Tropical\_T050&SubtropN\_AEROD\_v&31&1.20E-04&1.10E-04&4\\
SubtropN\_FLNTC&Tropical\_FLNTC&26&1.18E-04&7.40E-05&5\\
Tropical\_T050&Tropical\_FLNTC&1&1.16E-04&7.70E-05&5\\
Tropical\_T050&SubtropN\_AEROD\_v&6&1.14E-04&7.10E-05&5\\
Tropical\_T050&SubtropN\_FLNTC&26&1.14E-04&5.40E-05&5\\
SubtropN\_FLNTC&SubtropN\_AEROD\_v&16&1.12E-04&3.80E-05&5\\
Tropical\_AEROD\_v&Tropical\_FLNTC&1&1.10E-04&2.80E-05&5\\
SubtropN\_AEROD\_v&SubtropN\_T050&11&1.08E-04&1.03E-04&5\\
Tropical\_T050&Tropical\_FLNTC&26&1.07E-04&3.10E-05&4\\
SubtropN\_T050&SubtropN\_AEROD\_v&26&1.06E-04&4.30E-05&5\\
SubtropN\_FLNTC&SubtropN\_AEROD\_v&46&1.06E-04&6.40E-05&5\\
SubtropN\_T050&SubtropN\_AEROD\_v&31&1.06E-04&6.30E-05&5\\
Tropical\_AEROD\_v&Tropical\_FLNTC&36&1.06E-04&4.80E-05&5\\
SubtropN\_T050&Tropical\_T050&16&1.05E-04&7.50E-05&2\\
Tropical\_AEROD\_v&Tropical\_T050&16&1.05E-04&8.50E-05&2\\
SubtropN\_T050&Tropical\_FLNTC&16&1.05E-04&8.70E-05&4\\
Tropical\_FLNTC&SubtropN\_AEROD\_v&26&1.04E-04&2.70E-05&5\\
SubtropN\_AEROD\_v&Tropical\_AEROD\_v&21&1.03E-04&2.90E-05&3\\
SubtropN\_T050&SubtropN\_FLNTC&16&1.02E-04&2.90E-05&5\\
SubtropN\_T050&Tropical\_FLNTC&26&1.02E-04&8.40E-05&5\\
SubtropN\_FLNTC&SubtropN\_AEROD\_v&11&1.02E-04&4.40E-05&5\\
Tropical\_FLNTC&Tropical\_T050&11&1.00E-04&8.00E-05&2\\
Tropical\_FLNTC&Tropical\_T050&56&1.00E-04&0.00E+00&1\\
SubtropN\_AEROD\_v&Tropical\_FLNTC&11&1.00E-04&4.30E-05&5\\
SubtropN\_T050&SubtropN\_T050&26&9.80E-05&2.60E-05&5\\
SubtropN\_FLNTC&Tropical\_FLNTC&41&9.80E-05&2.50E-05&5\\
Tropical\_T050&Tropical\_FLNTC&51&9.80E-05&3.90E-05&5\\
SubtropN\_T050&Tropical\_FLNTC&6&9.60E-05&5.50E-05&5\\
Tropical\_T050&SubtropN\_AEROD\_v&26&9.60E-05&1.04E-04&5\\
SubtropN\_AEROD\_v&SubtropN\_T050&51&9.50E-05&7.80E-05&4\\
SubtropN\_FLNTC&Tropical\_T050&46&9.50E-05&5.00E-06&2\\
Tropical\_FLNTC&SubtropN\_T050&6&9.40E-05&6.30E-05&5\\
Tropical\_AEROD\_v&SubtropN\_T050&56&9.40E-05&6.00E-05&5\\
SubtropN\_T050&Tropical\_FLNTC&56&9.40E-05&8.20E-05&5\\
Tropical\_T050&SubtropN\_FLNTC&16&9.40E-05&6.30E-05&5\\
SubtropN\_AEROD\_v&Tropical\_FLNTC&46&9.40E-05&3.90E-05&5\\
Tropical\_FLNTC&SubtropN\_T050&51&9.40E-05&9.40E-05&5\\
SubtropN\_T050&Tropical\_T050&1&9.20E-05&1.20E-04&4\\
SubtropN\_T050&Tropical\_FLNTC&31&9.20E-05&5.80E-05&5\\
Tropical\_AEROD\_v&Tropical\_FLNTC&41&9.20E-05&8.20E-05&5\\
SubtropN\_T050&Tropical\_FLNTC&41&9.20E-05&4.70E-05&5\\
SubtropN\_T050&Tropical\_AEROD\_v&16&9.00E-05&9.20E-05&3\\
Tropical\_T050&SubtropN\_T050&26&9.00E-05&1.21E-04&5\\
Tropical\_T050&SubtropN\_T050&31&9.00E-05&8.00E-06&3\\
Tropical\_T050&Tropical\_AEROD\_v&36&9.00E-05&5.50E-05&4\\
SubtropN\_T050&SubtropN\_AEROD\_v&56&9.00E-05&5.20E-05&5\\
SubtropN\_AEROD\_v&Tropical\_FLNTC&21&8.80E-05&5.10E-05&5\\
Tropical\_T050&SubtropN\_AEROD\_v&36&8.80E-05&6.90E-05&5\\
SubtropN\_AEROD\_v&SubtropN\_T050&1&8.70E-05&5.20E-05&3\\
Tropical\_AEROD\_v&Tropical\_T050&56&8.70E-05&4.60E-05&3\\
Tropical\_FLNTC&Tropical\_FLNTC&36&8.60E-05&5.00E-05&5\\
SubtropN\_T050&Tropical\_FLNTC&1&8.60E-05&3.20E-05&5\\
SubtropN\_T050&Tropical\_AEROD\_v&51&8.50E-05&6.20E-05&4\\
SubtropN\_T050&SubtropN\_T050&31&8.40E-05&6.80E-05&5\\
SubtropN\_T050&SubtropN\_T050&11&8.20E-05&7.20E-05&5\\
Tropical\_T050&SubtropN\_T050&16&8.20E-05&6.50E-05&5\\
Tropical\_T050&Tropical\_FLNTC&46&8.20E-05&4.30E-05&5\\
Tropical\_AEROD\_v&Tropical\_FLNTC&51&8.20E-05&1.20E-05&5\\
Tropical\_T050&SubtropN\_AEROD\_v&21&8.20E-05&4.00E-05&5\\
SubtropN\_T050&SubtropN\_T050&51&8.00E-05&4.60E-05&4\\
Tropical\_FLNTC&Tropical\_T050&6&8.00E-05&0.00E+00&1\\
SubtropN\_T050&Tropical\_FLNTC&11&8.00E-05&3.20E-05&4\\
Tropical\_AEROD\_v&Tropical\_AEROD\_v&16&8.00E-05&7.90E-05&3\\
Tropical\_AEROD\_v&Tropical\_FLNTC&21&7.80E-05&2.40E-05&5\\
SubtropN\_T050&SubtropN\_T050&41&7.70E-05&1.20E-05&3\\
Tropical\_AEROD\_v&SubtropN\_T050&1&7.70E-05&1.70E-05&3\\
SubtropN\_T050&SubtropN\_T050&46&7.70E-05&3.90E-05&3\\
Tropical\_FLNTC&SubtropN\_T050&56&7.60E-05&7.80E-05&5\\
Tropical\_FLNTC&SubtropN\_T050&31&7.60E-05&5.00E-05&5\\
Tropical\_AEROD\_v&SubtropN\_T050&26&7.60E-05&6.60E-05&5\\
SubtropN\_FLNTC&SubtropN\_T050&36&7.40E-05&6.10E-05&5\\
Tropical\_T050&Tropical\_FLNTC&31&7.40E-05&3.00E-05&5\\
SubtropN\_T050&SubtropN\_AEROD\_v&41&7.40E-05&2.90E-05&5\\
Tropical\_T050&SubtropN\_AEROD\_v&1&7.40E-05&4.10E-05&5\\
Tropical\_T050&SubtropN\_AEROD\_v&41&7.40E-05&2.40E-05&5\\
SubtropN\_AEROD\_v&Tropical\_AEROD\_v&16&7.40E-05&7.00E-05&5\\
SubtropN\_T050&Tropical\_FLNTC&51&7.20E-05&5.00E-05&5\\
SubtropN\_AEROD\_v&Tropical\_AEROD\_v&1&7.00E-05&5.00E-05&2\\
SubtropN\_FLNTC&SubtropN\_T050&21&7.00E-05&7.20E-05&5\\
SubtropN\_T050&Tropical\_FLNTC&21&7.00E-05&3.10E-05&4\\
SubtropN\_FLNTC&Tropical\_AEROD\_v&21&7.00E-05&7.80E-05&3\\
SubtropN\_AEROD\_v&Tropical\_T050&16&7.00E-05&0.00E+00&1\\
SubtropN\_AEROD\_v&Tropical\_T050&11&7.00E-05&0.00E+00&1\\
Tropical\_AEROD\_v&Tropical\_T050&26&7.00E-05&0.00E+00&1\\
Tropical\_T050&Tropical\_FLNTC&6&7.00E-05&3.80E-05&5\\
Tropical\_T050&SubtropN\_T050&1&7.00E-05&5.20E-05&5\\
SubtropN\_AEROD\_v&SubtropN\_T050&36&6.60E-05&4.70E-05&5\\
SubtropN\_FLNTC&SubtropN\_T050&1&6.60E-05&4.30E-05&5\\
Tropical\_FLNTC&Tropical\_AEROD\_v&46&6.50E-05&6.20E-05&4\\
Tropical\_FLNTC&Tropical\_T050&16&6.50E-05&5.00E-06&2\\
Tropical\_FLNTC&SubtropN\_T050&11&6.30E-05&4.00E-05&4\\
Tropical\_FLNTC&SubtropN\_T050&26&6.20E-05&2.90E-05&5\\
SubtropN\_AEROD\_v&SubtropN\_T050&56&6.20E-05&2.00E-05&5\\
SubtropN\_FLNTC&Tropical\_T050&11&6.00E-05&0.00E+00&1\\
SubtropN\_T050&SubtropN\_T050&36&6.00E-05&5.40E-05&5\\
Tropical\_T050&Tropical\_T050&16&5.80E-05&6.10E-05&4\\
Tropical\_T050&Tropical\_AEROD\_v&1&5.70E-05&1.70E-05&3\\
SubtropN\_FLNTC&SubtropN\_T050&31&5.70E-05&1.70E-05&3\\
Tropical\_T050&Tropical\_AEROD\_v&56&5.60E-05&4.80E-05&5\\
SubtropN\_AEROD\_v&SubtropN\_T050&26&5.50E-05&3.60E-05&4\\
Tropical\_AEROD\_v&Tropical\_AEROD\_v&36&5.20E-05&1.30E-05&4\\
Tropical\_FLNTC&Tropical\_AEROD\_v&6&5.20E-05&4.60E-05&5\\
Tropical\_T050&Tropical\_AEROD\_v&51&5.20E-05&4.20E-05&5\\
SubtropN\_FLNTC&SubtropN\_T050&6&5.20E-05&3.70E-05&5\\
Tropical\_FLNTC&Tropical\_AEROD\_v&31&5.20E-05&4.90E-05&5\\
Tropical\_FLNTC&Tropical\_T050&41&5.00E-05&0.00E+00&1\\
Tropical\_AEROD\_v&Tropical\_T050&36&5.00E-05&4.00E-05&2\\
Tropical\_AEROD\_v&Tropical\_T050&21&5.00E-05&3.00E-05&2\\
Tropical\_T050&Tropical\_T050&31&5.00E-05&0.00E+00&1\\
Tropical\_FLNTC&Tropical\_AEROD\_v&36&5.00E-05&4.00E-05&2\\
SubtropN\_FLNTC&SubtropN\_T050&26&5.00E-05&5.80E-05&4\\
SubtropN\_FLNTC&SubtropN\_T050&46&4.80E-05&2.90E-05&5\\
Tropical\_T050&Tropical\_FLNTC&16&4.80E-05&2.10E-05&5\\
Tropical\_AEROD\_v&SubtropN\_T050&11&4.80E-05&2.90E-05&5\\
SubtropN\_T050&SubtropN\_T050&21&4.80E-05&1.80E-05&5\\
Tropical\_FLNTC&Tropical\_AEROD\_v&16&4.70E-05&2.90E-05&3\\
SubtropN\_FLNTC&Tropical\_AEROD\_v&41&4.60E-05&3.80E-05&5\\
Tropical\_AEROD\_v&Tropical\_FLNTC&46&4.60E-05&1.00E-05&5\\
Tropical\_FLNTC&Tropical\_AEROD\_v&21&4.50E-05&2.50E-05&4\\
SubtropN\_AEROD\_v&Tropical\_T050&56&4.50E-05&1.50E-05&2\\
Tropical\_T050&Tropical\_FLNTC&56&4.50E-05&3.00E-05&4\\
SubtropN\_FLNTC&SubtropN\_T050&51&4.50E-05&2.60E-05&4\\
SubtropN\_T050&Tropical\_AEROD\_v&46&4.40E-05&1.20E-05&5\\
Tropical\_T050&Tropical\_AEROD\_v&26&4.30E-05&2.90E-05&3\\
Tropical\_FLNTC&Tropical\_AEROD\_v&41&4.30E-05&2.60E-05&4\\
Tropical\_FLNTC&SubtropN\_T050&46&4.20E-05&2.00E-05&5\\
SubtropN\_T050&SubtropN\_T050&16&4.20E-05&2.10E-05&5\\
Tropical\_T050&Tropical\_AEROD\_v&31&4.00E-05&2.50E-05&4\\
SubtropN\_FLNTC&Tropical\_AEROD\_v&46&4.00E-05&2.90E-05&3\\
Tropical\_FLNTC&Tropical\_AEROD\_v&26&4.00E-05&3.60E-05&3\\
Tropical\_AEROD\_v&Tropical\_AEROD\_v&11&4.00E-05&0.00E+00&1\\
Tropical\_AEROD\_v&SubtropN\_T050&21&4.00E-05&1.40E-05&4\\
SubtropN\_T050&Tropical\_T050&46&4.00E-05&1.00E-05&2\\
Tropical\_AEROD\_v&SubtropN\_T050&41&3.80E-05&1.80E-05&4\\
Tropical\_FLNTC&Tropical\_AEROD\_v&51&3.80E-05&2.30E-05&4\\
SubtropN\_T050&Tropical\_T050&41&3.80E-05&3.30E-05&4\\
SubtropN\_AEROD\_v&Tropical\_AEROD\_v&56&3.70E-05&5.00E-06&3\\
Tropical\_T050&Tropical\_T050&11&3.70E-05&9.00E-06&3\\
SubtropN\_T050&Tropical\_AEROD\_v&6&3.60E-05&2.20E-05&5\\
SubtropN\_FLNTC&Tropical\_T050&1&3.50E-05&1.50E-05&2\\
SubtropN\_AEROD\_v&Tropical\_T050&41&3.50E-05&5.00E-06&2\\
SubtropN\_T050&Tropical\_T050&31&3.50E-05&1.80E-05&4\\
Tropical\_AEROD\_v&SubtropN\_T050&6&3.50E-05&9.00E-06&4\\
SubtropN\_AEROD\_v&SubtropN\_T050&41&3.50E-05&1.50E-05&2\\
Tropical\_T050&SubtropN\_T050&56&3.50E-05&1.80E-05&4\\
SubtropN\_AEROD\_v&SubtropN\_T050&21&3.40E-05&2.10E-05&5\\
Tropical\_T050&Tropical\_T050&6&3.30E-05&2.10E-05&3\\
SubtropN\_FLNTC&SubtropN\_T050&56&3.30E-05&1.70E-05&3\\
SubtropN\_FLNTC&Tropical\_AEROD\_v&51&3.30E-05&2.80E-05&4\\
SubtropN\_AEROD\_v&Tropical\_AEROD\_v&6&3.30E-05&2.50E-05&4\\
SubtropN\_FLNTC&Tropical\_AEROD\_v&31&3.30E-05&1.50E-05&4\\
Tropical\_FLNTC&SubtropN\_T050&1&3.30E-05&1.30E-05&4\\
Tropical\_AEROD\_v&Tropical\_AEROD\_v&21&3.30E-05&1.80E-05&4\\
SubtropN\_FLNTC&Tropical\_AEROD\_v&11&3.30E-05&1.50E-05&4\\
SubtropN\_FLNTC&SubtropN\_T050&41&3.20E-05&7.00E-06&5\\
Tropical\_AEROD\_v&SubtropN\_T050&51&3.20E-05&2.40E-05&5\\
SubtropN\_T050&Tropical\_AEROD\_v&26&3.00E-05&1.20E-05&4\\
SubtropN\_FLNTC&Tropical\_T050&6&3.00E-05&1.00E-05&2\\
SubtropN\_AEROD\_v&Tropical\_AEROD\_v&31&3.00E-05&1.20E-05&4\\
SubtropN\_FLNTC&Tropical\_T050&16&3.00E-05&1.00E-05&2\\
SubtropN\_FLNTC&Tropical\_T050&41&3.00E-05&1.00E-05&2\\
Tropical\_AEROD\_v&Tropical\_AEROD\_v&6&3.00E-05&1.20E-05&4\\
Tropical\_AEROD\_v&Tropical\_AEROD\_v&31&3.00E-05&0.00E+00&1\\
Tropical\_AEROD\_v&Tropical\_AEROD\_v&46&3.00E-05&0.00E+00&2\\
Tropical\_FLNTC&Tropical\_T050&51&3.00E-05&1.40E-05&3\\
SubtropN\_AEROD\_v&Tropical\_AEROD\_v&41&3.00E-05&2.30E-05&4\\
Tropical\_AEROD\_v&Tropical\_AEROD\_v&51&2.80E-05&1.80E-05&4\\
SubtropN\_FLNTC&SubtropN\_T050&11&2.70E-05&1.20E-05&3\\
SubtropN\_T050&Tropical\_T050&36&2.70E-05&5.00E-06&3\\
SubtropN\_AEROD\_v&SubtropN\_T050&46&2.70E-05&1.20E-05&3\\
Tropical\_FLNTC&Tropical\_T050&21&2.70E-05&1.20E-05&3\\
SubtropN\_T050&Tropical\_T050&21&2.70E-05&1.70E-05&3\\
SubtropN\_FLNTC&SubtropN\_T050&16&2.60E-05&1.50E-05&5\\
SubtropN\_T050&Tropical\_AEROD\_v&31&2.50E-05&1.10E-05&4\\
SubtropN\_AEROD\_v&Tropical\_T050&36&2.50E-05&5.00E-06&2\\
Tropical\_T050&Tropical\_T050&51&2.50E-05&1.50E-05&2\\
Tropical\_FLNTC&Tropical\_T050&46&2.50E-05&5.00E-06&2\\
Tropical\_AEROD\_v&Tropical\_T050&6&2.50E-05&1.50E-05&2\\
SubtropN\_FLNTC&Tropical\_AEROD\_v&1&2.50E-05&5.00E-06&2\\
Tropical\_T050&Tropical\_T050&26&2.50E-05&1.10E-05&4\\
Tropical\_FLNTC&Tropical\_T050&36&2.50E-05&5.00E-06&2\\
SubtropN\_AEROD\_v&Tropical\_AEROD\_v&26&2.50E-05&5.00E-06&2\\
Tropical\_AEROD\_v&SubtropN\_T050&36&2.40E-05&1.20E-05&5\\
SubtropN\_T050&Tropical\_AEROD\_v&1&2.40E-05&2.00E-05&5\\
Tropical\_AEROD\_v&Tropical\_AEROD\_v&56&2.30E-05&5.00E-06&3\\
SubtropN\_AEROD\_v&Tropical\_T050&21&2.30E-05&5.00E-06&3\\
SubtropN\_AEROD\_v&Tropical\_AEROD\_v&11&2.30E-05&1.10E-05&4\\
Tropical\_FLNTC&Tropical\_AEROD\_v&11&2.30E-05&1.30E-05&4\\
Tropical\_T050&Tropical\_AEROD\_v&46&2.30E-05&2.20E-05&4\\
SubtropN\_FLNTC&Tropical\_T050&36&2.00E-05&0.00E+00&1\\
Tropical\_FLNTC&Tropical\_T050&1&2.00E-05&8.00E-06&3\\
SubtropN\_FLNTC&Tropical\_T050&56&2.00E-05&1.00E-05&2\\
Tropical\_AEROD\_v&Tropical\_T050&41&2.00E-05&8.00E-06&3\\
Tropical\_T050&Tropical\_T050&41&2.00E-05&1.70E-05&4\\
SubtropN\_T050&Tropical\_AEROD\_v&41&2.00E-05&0.00E+00&2\\
Tropical\_T050&Tropical\_T050&21&2.00E-05&7.00E-06&4\\
SubtropN\_FLNTC&Tropical\_T050&51&2.00E-05&0.00E+00&1\\
SubtropN\_T050&Tropical\_T050&51&2.00E-05&1.00E-05&2\\
SubtropN\_AEROD\_v&SubtropN\_T050&6&2.00E-05&1.00E-05&2\\
SubtropN\_T050&Tropical\_AEROD\_v&56&2.00E-05&1.00E-05&2\\
SubtropN\_FLNTC&Tropical\_AEROD\_v&36&2.00E-05&8.00E-06&3\\
SubtropN\_T050&Tropical\_AEROD\_v&36&2.00E-05&8.00E-06&3\\
SubtropN\_AEROD\_v&Tropical\_AEROD\_v&36&2.00E-05&0.00E+00&2\\
SubtropN\_FLNTC&Tropical\_T050&21&2.00E-05&1.00E-05&2\\
Tropical\_AEROD\_v&Tropical\_AEROD\_v&26&2.00E-05&1.00E-05&2\\
Tropical\_AEROD\_v&Tropical\_T050&31&2.00E-05&0.00E+00&1\\
SubtropN\_AEROD\_v&Tropical\_T050&26&2.00E-05&1.00E-05&2\\
SubtropN\_FLNTC&Tropical\_T050&26&1.80E-05&8.00E-06&4\\
Tropical\_FLNTC&SubtropN\_T050&21&1.80E-05&4.00E-06&4\\
SubtropN\_AEROD\_v&Tropical\_AEROD\_v&46&1.80E-05&1.30E-05&4\\
Tropical\_FLNTC&Tropical\_T050&31&1.70E-05&5.00E-06&3\\
SubtropN\_T050&Tropical\_AEROD\_v&11&1.70E-05&5.00E-06&3\\
SubtropN\_AEROD\_v&SubtropN\_T050&16&1.60E-05&8.00E-06&5\\
SubtropN\_AEROD\_v&Tropical\_AEROD\_v&51&1.50E-05&5.00E-06&2\\
Tropical\_FLNTC&Tropical\_AEROD\_v&56&1.50E-05&5.00E-06&2\\
Tropical\_AEROD\_v&Tropical\_AEROD\_v&41&1.50E-05&5.00E-06&2\\
SubtropN\_T050&Tropical\_T050&6&1.50E-05&5.00E-06&2\\
Tropical\_AEROD\_v&Tropical\_T050&51&1.30E-05&5.00E-06&3\\
SubtropN\_AEROD\_v&Tropical\_T050&51&1.00E-05&0.00E+00&1\\
Tropical\_FLNTC&Tropical\_T050&26&1.00E-05&0.00E+00&2\\
Tropical\_AEROD\_v&Tropical\_T050&46&1.00E-05&0.00E+00&1\\
SubtropN\_AEROD\_v&Tropical\_T050&31&1.00E-05&0.00E+00&2\\
SubtropN\_T050&Tropical\_T050&26&1.00E-05&0.00E+00&1\\
SubtropN\_AEROD\_v&Tropical\_T050&6&1.00E-05&0.00E+00&1\\
SubtropN\_FLNTC&Tropical\_AEROD\_v&6&1.00E-05&0.00E+00&2\\
SubtropN\_AEROD\_v&Tropical\_T050&46&1.00E-05&0.00E+00&1\\
\hline
\end{longtblr}

\subsection*{A.4.  Regional Surface}
\begin{longtblr}[
  caption = {Mount Pinatubo exemplar: unpruned pathway edge weights and their standard deviations for the surface warming pathway obtained using zonally-averaged data windowed to 750 days.},
  label = {tab:app_tropics_surf},
]{
  colspec = {llcccc},
  width=\textwidth,rowsep=0pt,
  cells={font=\small},
  rowhead = 2,
} 

    \hline \hline
        \multirow{2}{*}{\textbf{Source}} & \multirow{2}{*}{\textbf{Target}} & \textbf{Lag } & \textbf{SHAP }& \textbf{Weight }&\textbf{Ensembles }\\
   & &{\bf (days)} &{\bf Weight} & $\sigma$ & {\bf with edge} \\
        \hline
SubtropN\_TREFHT&SubtropN\_TREFHT&1&1.75E-01&1.29E-02&5\\
Tropical\_AEROD\_v&Tropical\_AEROD\_v&1&1.57E-01&2.02E-02&5\\
SubtropN\_FSDSC&SubtropN\_FSDSC&1&1.44E-01&2.05E-02&5\\
SubtropN\_AEROD\_v&SubtropN\_AEROD\_v&1&1.40E-01&2.23E-02&5\\
Tropical\_FSDSC&Tropical\_FSDSC&1&1.38E-01&3.25E-02&5\\
Tropical\_TREFHT&Tropical\_TREFHT&1&6.85E-02&1.79E-02&5\\
Tropical\_AEROD\_v&Tropical\_FSDSC&1&3.86E-03&2.18E-03&5\\
Tropical\_FSDSC&Tropical\_AEROD\_v&1&2.08E-03&1.43E-03&5\\
SubtropN\_AEROD\_v&SubtropN\_FSDSC&1&9.66E-04&4.42E-04&5\\
SubtropN\_AEROD\_v&SubtropN\_FSDSC&11&8.64E-04&8.28E-04&5\\
SubtropN\_FSDSC&SubtropN\_TREFHT&1&8.50E-04&4.42E-04&5\\
SubtropN\_TREFHT&SubtropN\_TREFHT&26&8.30E-04&5.24E-04&5\\
Tropical\_TREFHT&SubtropN\_TREFHT&6&7.22E-04&5.26E-04&5\\
SubtropN\_TREFHT&SubtropN\_TREFHT&46&7.08E-04&5.91E-04&5\\
SubtropN\_TREFHT&SubtropN\_TREFHT&56&6.66E-04&4.62E-04&5\\
SubtropN\_TREFHT&SubtropN\_TREFHT&31&6.60E-04&4.56E-04&5\\
SubtropN\_TREFHT&SubtropN\_TREFHT&11&6.44E-04&2.58E-04&5\\
Tropical\_TREFHT&SubtropN\_TREFHT&11&6.38E-04&3.92E-04&5\\
Tropical\_TREFHT&SubtropN\_AEROD\_v&16&6.32E-04&5.42E-04&5\\
SubtropN\_AEROD\_v&SubtropN\_TREFHT&11&6.10E-04&2.66E-04&5\\
SubtropN\_AEROD\_v&SubtropN\_TREFHT&1&6.10E-04&3.69E-04&5\\
Tropical\_TREFHT&SubtropN\_TREFHT&1&5.90E-04&4.95E-04&5\\
Tropical\_TREFHT&SubtropN\_TREFHT&36&5.90E-04&5.73E-04&5\\
SubtropN\_AEROD\_v&SubtropN\_TREFHT&16&5.84E-04&4.93E-04&5\\
SubtropN\_TREFHT&SubtropN\_TREFHT&36&5.52E-04&3.60E-04&5\\
Tropical\_TREFHT&SubtropN\_TREFHT&51&5.30E-04&2.03E-04&5\\
SubtropN\_AEROD\_v&SubtropN\_TREFHT&51&5.26E-04&6.70E-04&5\\
SubtropN\_TREFHT&SubtropN\_TREFHT&21&5.08E-04&2.65E-04&5\\
Tropical\_TREFHT&SubtropN\_TREFHT&26&5.06E-04&2.57E-04&5\\
SubtropN\_AEROD\_v&SubtropN\_TREFHT&26&4.92E-04&2.93E-04&5\\
Tropical\_AEROD\_v&SubtropN\_AEROD\_v&6&4.74E-04&3.99E-04&5\\
SubtropN\_TREFHT&SubtropN\_AEROD\_v&1&4.56E-04&3.93E-04&5\\
SubtropN\_FSDSC&SubtropN\_TREFHT&21&4.46E-04&1.45E-04&5\\
SubtropN\_TREFHT&SubtropN\_TREFHT&51&4.28E-04&2.29E-04&5\\
SubtropN\_TREFHT&SubtropN\_TREFHT&16&4.24E-04&2.84E-04&5\\
SubtropN\_FSDSC&SubtropN\_TREFHT&16&4.22E-04&3.63E-04&5\\
Tropical\_TREFHT&SubtropN\_TREFHT&41&4.18E-04&2.51E-04&5\\
SubtropN\_AEROD\_v&SubtropN\_FSDSC&31&4.04E-04&1.99E-04&5\\
SubtropN\_FSDSC&SubtropN\_TREFHT&26&3.98E-04&3.16E-04&5\\
SubtropN\_FSDSC&SubtropN\_TREFHT&41&3.94E-04&5.50E-05&5\\
SubtropN\_AEROD\_v&SubtropN\_TREFHT&21&3.94E-04&2.97E-04&5\\
Tropical\_AEROD\_v&SubtropN\_TREFHT&6&3.94E-04&4.13E-04&5\\
SubtropN\_TREFHT&SubtropN\_TREFHT&6&3.90E-04&2.30E-04&5\\
SubtropN\_FSDSC&SubtropN\_FSDSC&16&3.86E-04&2.99E-04&5\\
Tropical\_FSDSC&SubtropN\_AEROD\_v&6&3.68E-04&2.59E-04&5\\
Tropical\_TREFHT&SubtropN\_TREFHT&16&3.68E-04&1.48E-04&5\\
SubtropN\_TREFHT&SubtropN\_AEROD\_v&16&3.64E-04&3.61E-04&5\\
Tropical\_TREFHT&SubtropN\_TREFHT&56&3.60E-04&2.11E-04&5\\
SubtropN\_FSDSC&SubtropN\_TREFHT&36&3.60E-04&2.16E-04&5\\
Tropical\_FSDSC&SubtropN\_TREFHT&21&3.54E-04&3.43E-04&5\\
SubtropN\_FSDSC&SubtropN\_FSDSC&6&3.52E-04&8.50E-05&5\\
Tropical\_TREFHT&SubtropN\_FSDSC&41&3.50E-04&3.37E-04&5\\
SubtropN\_AEROD\_v&SubtropN\_FSDSC&26&3.48E-04&2.68E-04&5\\
Tropical\_AEROD\_v&SubtropN\_FSDSC&36&3.38E-04&2.10E-04&5\\
Tropical\_AEROD\_v&SubtropN\_TREFHT&1&3.32E-04&2.81E-04&5\\
Tropical\_TREFHT&SubtropN\_FSDSC&31&3.30E-04&3.16E-04&5\\
Tropical\_TREFHT&SubtropN\_TREFHT&46&3.28E-04&2.64E-04&5\\
Tropical\_FSDSC&SubtropN\_FSDSC&6&3.24E-04&2.20E-04&5\\
SubtropN\_TREFHT&SubtropN\_FSDSC&56&3.22E-04&9.60E-05&5\\
Tropical\_AEROD\_v&SubtropN\_TREFHT&26&3.18E-04&3.21E-04&5\\
Tropical\_TREFHT&SubtropN\_FSDSC&46&3.16E-04&1.92E-04&5\\
SubtropN\_TREFHT&SubtropN\_FSDSC&1&3.14E-04&1.63E-04&5\\
SubtropN\_AEROD\_v&SubtropN\_AEROD\_v&11&3.12E-04&1.73E-04&5\\
Tropical\_TREFHT&SubtropN\_FSDSC&6&3.08E-04&2.68E-04&5\\
SubtropN\_TREFHT&SubtropN\_AEROD\_v&26&3.08E-04&1.95E-04&5\\
SubtropN\_FSDSC&SubtropN\_AEROD\_v&1&3.08E-04&1.21E-04&5\\
Tropical\_FSDSC&SubtropN\_TREFHT&31&3.04E-04&2.52E-04&5\\
SubtropN\_TREFHT&SubtropN\_FSDSC&21&3.04E-04&2.01E-04&5\\
Tropical\_FSDSC&SubtropN\_TREFHT&56&3.02E-04&1.99E-04&5\\
SubtropN\_TREFHT&SubtropN\_FSDSC&41&3.00E-04&2.02E-04&5\\
SubtropN\_FSDSC&SubtropN\_FSDSC&51&3.00E-04&3.18E-04&4\\
Tropical\_TREFHT&SubtropN\_TREFHT&21&2.96E-04&2.75E-04&5\\
SubtropN\_FSDSC&SubtropN\_FSDSC&11&2.94E-04&1.76E-04&5\\
SubtropN\_TREFHT&SubtropN\_TREFHT&41&2.94E-04&1.54E-04&5\\
SubtropN\_AEROD\_v&SubtropN\_FSDSC&6&2.94E-04&1.68E-04&5\\
SubtropN\_TREFHT&SubtropN\_FSDSC&11&2.88E-04&1.46E-04&5\\
Tropical\_AEROD\_v&SubtropN\_FSDSC&6&2.86E-04&1.19E-04&5\\
Tropical\_TREFHT&SubtropN\_AEROD\_v&31&2.86E-04&2.10E-04&5\\
SubtropN\_TREFHT&Tropical\_TREFHT&1&2.84E-04&2.82E-04&5\\
SubtropN\_TREFHT&SubtropN\_FSDSC&16&2.80E-04&1.68E-04&5\\
Tropical\_FSDSC&SubtropN\_TREFHT&46&2.78E-04&1.79E-04&5\\
Tropical\_TREFHT&SubtropN\_AEROD\_v&11&2.78E-04&1.84E-04&5\\
SubtropN\_AEROD\_v&SubtropN\_AEROD\_v&16&2.78E-04&1.46E-04&5\\
SubtropN\_TREFHT&SubtropN\_AEROD\_v&31&2.78E-04&3.17E-04&5\\
Tropical\_TREFHT&SubtropN\_AEROD\_v&51&2.78E-04&1.65E-04&5\\
SubtropN\_FSDSC&SubtropN\_TREFHT&51&2.76E-04&2.27E-04&5\\
SubtropN\_AEROD\_v&SubtropN\_TREFHT&41&2.76E-04&1.52E-04&5\\
SubtropN\_AEROD\_v&SubtropN\_AEROD\_v&6&2.74E-04&1.68E-04&5\\
SubtropN\_AEROD\_v&SubtropN\_FSDSC&56&2.68E-04&8.80E-05&5\\
SubtropN\_FSDSC&SubtropN\_FSDSC&46&2.68E-04&1.78E-04&5\\
SubtropN\_TREFHT&SubtropN\_FSDSC&46&2.68E-04&1.22E-04&5\\
SubtropN\_FSDSC&SubtropN\_FSDSC&41&2.66E-04&1.60E-04&5\\
Tropical\_TREFHT&SubtropN\_FSDSC&1&2.64E-04&1.50E-04&5\\
SubtropN\_FSDSC&SubtropN\_AEROD\_v&51&2.64E-04&1.28E-04&5\\
Tropical\_TREFHT&SubtropN\_AEROD\_v&21&2.64E-04&2.71E-04&5\\
SubtropN\_FSDSC&SubtropN\_FSDSC&31&2.60E-04&1.18E-04&5\\
Tropical\_TREFHT&SubtropN\_FSDSC&16&2.60E-04&1.86E-04&5\\
SubtropN\_AEROD\_v&SubtropN\_AEROD\_v&46&2.58E-04&2.27E-04&5\\
Tropical\_TREFHT&SubtropN\_FSDSC&51&2.58E-04&1.12E-04&5\\
Tropical\_FSDSC&SubtropN\_AEROD\_v&26&2.56E-04&2.90E-04&5\\
Tropical\_TREFHT&SubtropN\_AEROD\_v&46&2.54E-04&1.44E-04&5\\
SubtropN\_AEROD\_v&SubtropN\_TREFHT&6&2.50E-04&9.20E-05&5\\
SubtropN\_AEROD\_v&SubtropN\_FSDSC&16&2.50E-04&1.83E-04&5\\
SubtropN\_AEROD\_v&SubtropN\_FSDSC&21&2.50E-04&7.80E-05&5\\
SubtropN\_AEROD\_v&SubtropN\_TREFHT&36&2.44E-04&1.32E-04&5\\
Tropical\_TREFHT&SubtropN\_FSDSC&56&2.44E-04&5.90E-05&5\\
Tropical\_FSDSC&SubtropN\_TREFHT&26&2.42E-04&1.96E-04&5\\
Tropical\_FSDSC&SubtropN\_FSDSC&26&2.40E-04&1.42E-04&5\\
Tropical\_FSDSC&SubtropN\_TREFHT&16&2.40E-04&1.63E-04&5\\
Tropical\_AEROD\_v&SubtropN\_FSDSC&41&2.40E-04&1.27E-04&4\\
SubtropN\_FSDSC&SubtropN\_FSDSC&56&2.36E-04&1.22E-04&5\\
Tropical\_AEROD\_v&SubtropN\_TREFHT&41&2.33E-04&1.79E-04&4\\
SubtropN\_AEROD\_v&SubtropN\_AEROD\_v&36&2.32E-04&1.61E-04&5\\
SubtropN\_FSDSC&SubtropN\_TREFHT&46&2.32E-04&1.10E-04&5\\
SubtropN\_TREFHT&SubtropN\_AEROD\_v&46&2.26E-04&2.13E-04&5\\
SubtropN\_TREFHT&SubtropN\_FSDSC&51&2.26E-04&1.42E-04&5\\
Tropical\_TREFHT&SubtropN\_TREFHT&31&2.26E-04&6.40E-05&5\\
Tropical\_FSDSC&SubtropN\_AEROD\_v&21&2.26E-04&2.29E-04&5\\
SubtropN\_AEROD\_v&SubtropN\_AEROD\_v&21&2.24E-04&1.35E-04&5\\
SubtropN\_FSDSC&SubtropN\_FSDSC&26&2.24E-04&1.04E-04&5\\
Tropical\_TREFHT&Tropical\_TREFHT&26&2.22E-04&8.50E-05&5\\
SubtropN\_FSDSC&SubtropN\_TREFHT&6&2.22E-04&1.02E-04&5\\
Tropical\_FSDSC&SubtropN\_TREFHT&41&2.20E-04&2.12E-04&5\\
SubtropN\_TREFHT&SubtropN\_FSDSC&36&2.20E-04&4.80E-05&5\\
Tropical\_FSDSC&SubtropN\_TREFHT&36&2.18E-04&9.90E-05&5\\
Tropical\_AEROD\_v&SubtropN\_AEROD\_v&11&2.18E-04&1.46E-04&5\\
Tropical\_AEROD\_v&SubtropN\_AEROD\_v&36&2.14E-04&1.41E-04&5\\
Tropical\_TREFHT&SubtropN\_FSDSC&21&2.14E-04&1.28E-04&5\\
SubtropN\_TREFHT&SubtropN\_AEROD\_v&56&2.12E-04&1.24E-04&5\\
SubtropN\_AEROD\_v&SubtropN\_TREFHT&46&2.12E-04&1.56E-04&5\\
SubtropN\_FSDSC&SubtropN\_AEROD\_v&31&2.12E-04&1.54E-04&5\\
SubtropN\_FSDSC&SubtropN\_AEROD\_v&16&2.12E-04&1.31E-04&5\\
Tropical\_FSDSC&SubtropN\_TREFHT&6&2.10E-04&8.90E-05&5\\
Tropical\_FSDSC&SubtropN\_TREFHT&11&2.08E-04&1.49E-04&5\\
Tropical\_FSDSC&SubtropN\_AEROD\_v&36&2.07E-04&1.48E-04&4\\
Tropical\_TREFHT&SubtropN\_AEROD\_v&26&2.06E-04&1.39E-04&5\\
SubtropN\_FSDSC&SubtropN\_TREFHT&56&2.06E-04&8.00E-05&5\\
SubtropN\_TREFHT&SubtropN\_FSDSC&31&2.04E-04&4.10E-05&5\\
Tropical\_AEROD\_v&SubtropN\_FSDSC&16&2.04E-04&2.14E-04&5\\
SubtropN\_AEROD\_v&SubtropN\_AEROD\_v&56&2.04E-04&1.73E-04&5\\
Tropical\_TREFHT&SubtropN\_AEROD\_v&1&2.02E-04&1.65E-04&5\\
Tropical\_AEROD\_v&SubtropN\_TREFHT&21&2.00E-04&5.80E-05&5\\
SubtropN\_TREFHT&SubtropN\_FSDSC&6&2.00E-04&4.90E-05&5\\
SubtropN\_FSDSC&SubtropN\_TREFHT&11&1.98E-04&1.09E-04&5\\
SubtropN\_AEROD\_v&SubtropN\_TREFHT&56&1.98E-04&1.36E-04&5\\
Tropical\_FSDSC&SubtropN\_AEROD\_v&31&1.98E-04&1.61E-04&5\\
Tropical\_TREFHT&SubtropN\_AEROD\_v&56&1.96E-04&9.50E-05&5\\
Tropical\_FSDSC&Tropical\_FSDSC&26&1.90E-04&2.55E-04&3\\
Tropical\_AEROD\_v&SubtropN\_FSDSC&21&1.90E-04&1.48E-04&5\\
Tropical\_AEROD\_v&SubtropN\_AEROD\_v&26&1.90E-04&8.90E-05&5\\
SubtropN\_AEROD\_v&Tropical\_TREFHT&1&1.90E-04&2.17E-04&5\\
SubtropN\_FSDSC&SubtropN\_AEROD\_v&11&1.88E-04&1.14E-04&5\\
Tropical\_TREFHT&SubtropN\_AEROD\_v&41&1.88E-04&1.91E-04&5\\
Tropical\_TREFHT&SubtropN\_FSDSC&26&1.86E-04&1.16E-04&5\\
Tropical\_AEROD\_v&SubtropN\_FSDSC&11&1.84E-04&9.20E-05&5\\
Tropical\_FSDSC&Tropical\_AEROD\_v&21&1.83E-04&1.83E-04&3\\
SubtropN\_FSDSC&SubtropN\_FSDSC&21&1.82E-04&1.62E-04&5\\
Tropical\_TREFHT&SubtropN\_FSDSC&11&1.82E-04&6.80E-05&5\\
Tropical\_AEROD\_v&SubtropN\_TREFHT&11&1.80E-04&1.67E-04&5\\
Tropical\_FSDSC&SubtropN\_FSDSC&11&1.78E-04&6.60E-05&5\\
Tropical\_FSDSC&SubtropN\_AEROD\_v&11&1.78E-04&8.30E-05&4\\
Tropical\_AEROD\_v&SubtropN\_AEROD\_v&16&1.76E-04&1.00E-04&5\\
Tropical\_AEROD\_v&SubtropN\_TREFHT&31&1.74E-04&8.40E-05&5\\
Tropical\_FSDSC&SubtropN\_TREFHT&51&1.73E-04&8.70E-05&4\\
SubtropN\_AEROD\_v&SubtropN\_FSDSC&36&1.72E-04&6.30E-05&5\\
Tropical\_FSDSC&SubtropN\_TREFHT&1&1.72E-04&1.17E-04&5\\
SubtropN\_AEROD\_v&SubtropN\_FSDSC&41&1.70E-04&1.08E-04&5\\
SubtropN\_FSDSC&SubtropN\_AEROD\_v&41&1.68E-04&1.13E-04&5\\
SubtropN\_AEROD\_v&SubtropN\_AEROD\_v&51&1.66E-04&1.15E-04&5\\
SubtropN\_AEROD\_v&SubtropN\_TREFHT&31&1.66E-04&4.60E-05&5\\
Tropical\_AEROD\_v&SubtropN\_AEROD\_v&46&1.66E-04&1.07E-04&5\\
SubtropN\_FSDSC&SubtropN\_AEROD\_v&6&1.64E-04&8.20E-05&5\\
Tropical\_AEROD\_v&SubtropN\_AEROD\_v&21&1.64E-04&1.61E-04&5\\
Tropical\_FSDSC&SubtropN\_FSDSC&36&1.64E-04&8.60E-05&5\\
Tropical\_TREFHT&SubtropN\_AEROD\_v&6&1.62E-04&8.00E-05&5\\
SubtropN\_FSDSC&SubtropN\_TREFHT&31&1.60E-04&6.90E-05&5\\
SubtropN\_AEROD\_v&SubtropN\_FSDSC&51&1.60E-04&1.17E-04&4\\
Tropical\_AEROD\_v&SubtropN\_AEROD\_v&51&1.58E-04&7.50E-05&5\\
Tropical\_FSDSC&SubtropN\_FSDSC&21&1.58E-04&9.20E-05&5\\
Tropical\_AEROD\_v&SubtropN\_TREFHT&16&1.58E-04&1.24E-04&5\\
SubtropN\_AEROD\_v&Tropical\_FSDSC&26&1.58E-04&1.55E-04&4\\
Tropical\_AEROD\_v&SubtropN\_AEROD\_v&41&1.56E-04&8.10E-05&5\\
Tropical\_FSDSC&SubtropN\_FSDSC&16&1.56E-04&1.27E-04&5\\
SubtropN\_TREFHT&SubtropN\_AEROD\_v&51&1.54E-04&1.31E-04&5\\
Tropical\_FSDSC&SubtropN\_AEROD\_v&16&1.53E-04&7.80E-05&4\\
SubtropN\_TREFHT&Tropical\_FSDSC&21&1.52E-04&1.17E-04&5\\
Tropical\_TREFHT&SubtropN\_FSDSC&36&1.52E-04&8.90E-05&5\\
Tropical\_FSDSC&SubtropN\_AEROD\_v&46&1.52E-04&1.25E-04&5\\
Tropical\_FSDSC&SubtropN\_FSDSC&1&1.52E-04&1.02E-04&5\\
Tropical\_FSDSC&SubtropN\_FSDSC&31&1.50E-04&8.40E-05&5\\
Tropical\_TREFHT&Tropical\_AEROD\_v&6&1.48E-04&1.82E-04&5\\
SubtropN\_AEROD\_v&SubtropN\_FSDSC&46&1.48E-04&7.80E-05&4\\
SubtropN\_FSDSC&SubtropN\_AEROD\_v&26&1.46E-04&1.21E-04&5\\
SubtropN\_FSDSC&SubtropN\_AEROD\_v&21&1.46E-04&7.80E-05&5\\
Tropical\_FSDSC&Tropical\_FSDSC&41&1.45E-04&1.35E-04&2\\
SubtropN\_TREFHT&SubtropN\_AEROD\_v&21&1.44E-04&1.07E-04&5\\
SubtropN\_TREFHT&SubtropN\_FSDSC&26&1.42E-04&4.50E-05&5\\
SubtropN\_TREFHT&Tropical\_TREFHT&36&1.42E-04&1.90E-04&5\\
SubtropN\_TREFHT&Tropical\_AEROD\_v&21&1.40E-04&1.18E-04&5\\
Tropical\_AEROD\_v&SubtropN\_AEROD\_v&31&1.40E-04&3.70E-05&5\\
SubtropN\_TREFHT&Tropical\_TREFHT&11&1.40E-04&1.66E-04&5\\
Tropical\_FSDSC&SubtropN\_AEROD\_v&51&1.40E-04&7.70E-05&5\\
SubtropN\_FSDSC&SubtropN\_AEROD\_v&56&1.38E-04&8.40E-05&5\\
SubtropN\_TREFHT&SubtropN\_AEROD\_v&6&1.38E-04&8.30E-05&5\\
SubtropN\_AEROD\_v&SubtropN\_AEROD\_v&41&1.35E-04&4.70E-05&4\\
Tropical\_FSDSC&SubtropN\_FSDSC&41&1.33E-04&3.80E-05&3\\
Tropical\_TREFHT&Tropical\_TREFHT&6&1.32E-04&5.60E-05&5\\
SubtropN\_FSDSC&SubtropN\_FSDSC&36&1.32E-04&1.17E-04&5\\
Tropical\_AEROD\_v&SubtropN\_FSDSC&56&1.30E-04&5.40E-05&4\\
Tropical\_AEROD\_v&Tropical\_FSDSC&6&1.30E-04&1.42E-04&3\\
Tropical\_AEROD\_v&SubtropN\_TREFHT&56&1.28E-04&5.90E-05&5\\
Tropical\_FSDSC&SubtropN\_AEROD\_v&1&1.28E-04&9.60E-05&5\\
Tropical\_AEROD\_v&SubtropN\_FSDSC&26&1.24E-04&6.40E-05&5\\
Tropical\_AEROD\_v&SubtropN\_FSDSC&31&1.22E-04&5.60E-05&5\\
Tropical\_AEROD\_v&SubtropN\_FSDSC&46&1.18E-04&6.80E-05&5\\
SubtropN\_AEROD\_v&SubtropN\_AEROD\_v&26&1.18E-04&7.10E-05&5\\
Tropical\_TREFHT&Tropical\_TREFHT&36&1.18E-04&3.40E-05&5\\
Tropical\_AEROD\_v&SubtropN\_AEROD\_v&56&1.18E-04&4.20E-05&4\\
Tropical\_AEROD\_v&SubtropN\_FSDSC&1&1.16E-04&1.07E-04&5\\
Tropical\_AEROD\_v&Tropical\_TREFHT&51&1.16E-04&1.40E-04&5\\
Tropical\_FSDSC&SubtropN\_FSDSC&56&1.15E-04&6.10E-05&4\\
SubtropN\_TREFHT&SubtropN\_AEROD\_v&41&1.14E-04&5.10E-05&5\\
Tropical\_AEROD\_v&SubtropN\_TREFHT&36&1.14E-04&5.50E-05&5\\
Tropical\_TREFHT&SubtropN\_AEROD\_v&36&1.12E-04&4.30E-05&5\\
SubtropN\_FSDSC&SubtropN\_AEROD\_v&46&1.10E-04&6.30E-05&5\\
Tropical\_FSDSC&SubtropN\_FSDSC&51&1.10E-04&3.70E-05&4\\
SubtropN\_AEROD\_v&SubtropN\_AEROD\_v&31&1.08E-04&3.40E-05&5\\
Tropical\_FSDSC&SubtropN\_FSDSC&46&1.08E-04&6.20E-05&5\\
Tropical\_FSDSC&SubtropN\_AEROD\_v&41&1.04E-04&6.30E-05&5\\
SubtropN\_FSDSC&Tropical\_TREFHT&31&1.02E-04&6.90E-05&5\\
SubtropN\_TREFHT&SubtropN\_AEROD\_v&36&1.00E-04&5.20E-05&5\\
Tropical\_AEROD\_v&SubtropN\_FSDSC&51&1.00E-04&8.20E-05&5\\
SubtropN\_AEROD\_v&Tropical\_TREFHT&36&9.80E-05&9.70E-05&5\\
SubtropN\_FSDSC&SubtropN\_AEROD\_v&36&9.80E-05&5.40E-05&5\\
SubtropN\_AEROD\_v&Tropical\_TREFHT&11&9.80E-05&8.20E-05&5\\
Tropical\_AEROD\_v&SubtropN\_TREFHT&51&9.70E-05&3.10E-05&4\\
SubtropN\_AEROD\_v&Tropical\_AEROD\_v&21&9.70E-05&3.10E-05&3\\
SubtropN\_AEROD\_v&Tropical\_TREFHT&31&9.60E-05&5.60E-05&5\\
Tropical\_FSDSC&Tropical\_TREFHT&16&9.60E-05&8.20E-05&5\\
Tropical\_TREFHT&Tropical\_TREFHT&51&9.60E-05&5.80E-05&5\\
Tropical\_TREFHT&Tropical\_TREFHT&56&9.60E-05&3.50E-05&5\\
SubtropN\_FSDSC&Tropical\_TREFHT&1&9.40E-05&4.50E-05&5\\
Tropical\_AEROD\_v&Tropical\_AEROD\_v&16&9.30E-05&1.31E-04&4\\
SubtropN\_TREFHT&Tropical\_FSDSC&36&9.20E-05&1.54E-04&5\\
SubtropN\_TREFHT&SubtropN\_AEROD\_v&11&9.00E-05&5.60E-05&5\\
SubtropN\_TREFHT&Tropical\_FSDSC&51&9.00E-05&0.00E+00&1\\
SubtropN\_TREFHT&Tropical\_FSDSC&1&8.80E-05&7.00E-05&5\\
SubtropN\_FSDSC&Tropical\_TREFHT&51&8.80E-05&8.40E-05&5\\
Tropical\_TREFHT&Tropical\_TREFHT&16&8.80E-05&3.50E-05&5\\
Tropical\_TREFHT&Tropical\_FSDSC&1&8.80E-05&6.40E-05&4\\
SubtropN\_AEROD\_v&Tropical\_TREFHT&26&8.60E-05&5.40E-05&5\\
Tropical\_TREFHT&Tropical\_TREFHT&31&8.40E-05&3.40E-05&5\\
SubtropN\_TREFHT&Tropical\_TREFHT&41&8.20E-05&6.80E-05&5\\
SubtropN\_FSDSC&Tropical\_TREFHT&16&8.20E-05&2.70E-05&5\\
SubtropN\_FSDSC&Tropical\_AEROD\_v&26&8.00E-05&1.10E-04&4\\
Tropical\_FSDSC&Tropical\_FSDSC&11&8.00E-05&7.10E-05&3\\
SubtropN\_TREFHT&Tropical\_TREFHT&21&7.80E-05&2.70E-05&5\\
SubtropN\_FSDSC&Tropical\_FSDSC&26&7.80E-05&1.11E-04&4\\
Tropical\_FSDSC&Tropical\_AEROD\_v&6&7.70E-05&8.40E-05&4\\
Tropical\_AEROD\_v&Tropical\_FSDSC&21&7.70E-05&9.00E-05&4\\
Tropical\_FSDSC&Tropical\_AEROD\_v&31&7.70E-05&8.00E-05&3\\
Tropical\_FSDSC&Tropical\_FSDSC&21&7.50E-05&5.60E-05&4\\
Tropical\_FSDSC&Tropical\_TREFHT&1&7.50E-05&5.00E-05&4\\
SubtropN\_TREFHT&Tropical\_TREFHT&56&7.40E-05&3.50E-05&5\\
Tropical\_AEROD\_v&Tropical\_TREFHT&26&7.40E-05&4.20E-05&5\\
SubtropN\_FSDSC&Tropical\_TREFHT&26&7.40E-05&5.50E-05&5\\
SubtropN\_FSDSC&Tropical\_TREFHT&36&7.40E-05&4.20E-05&5\\
SubtropN\_TREFHT&Tropical\_AEROD\_v&1&7.30E-05&7.50E-05&3\\
Tropical\_AEROD\_v&Tropical\_FSDSC&36&7.30E-05&5.40E-05&3\\
Tropical\_FSDSC&SubtropN\_AEROD\_v&56&7.20E-05&4.00E-05&5\\
Tropical\_AEROD\_v&SubtropN\_AEROD\_v&1&7.00E-05&4.50E-05&5\\
Tropical\_FSDSC&Tropical\_TREFHT&46&7.00E-05&5.50E-05&4\\
SubtropN\_TREFHT&Tropical\_FSDSC&31&7.00E-05&7.80E-05&3\\
Tropical\_AEROD\_v&Tropical\_AEROD\_v&36&7.00E-05&2.70E-05&4\\
SubtropN\_AEROD\_v&Tropical\_TREFHT&46&7.00E-05&2.60E-05&5\\
SubtropN\_AEROD\_v&Tropical\_AEROD\_v&16&7.00E-05&4.80E-05&4\\
Tropical\_TREFHT&Tropical\_TREFHT&21&6.80E-05&3.70E-05&5\\
Tropical\_TREFHT&Tropical\_FSDSC&56&6.80E-05&3.70E-05&5\\
SubtropN\_AEROD\_v&Tropical\_FSDSC&41&6.70E-05&2.50E-05&3\\
SubtropN\_TREFHT&Tropical\_TREFHT&26&6.60E-05&2.90E-05&5\\
Tropical\_TREFHT&Tropical\_TREFHT&11&6.60E-05&1.40E-05&5\\
SubtropN\_FSDSC&Tropical\_TREFHT&11&6.60E-05&5.70E-05&5\\
SubtropN\_FSDSC&Tropical\_FSDSC&46&6.50E-05&3.60E-05&4\\
Tropical\_AEROD\_v&Tropical\_FSDSC&31&6.50E-05&3.60E-05&4\\
Tropical\_FSDSC&Tropical\_AEROD\_v&26&6.50E-05&4.40E-05&4\\
Tropical\_TREFHT&Tropical\_TREFHT&41&6.40E-05&3.00E-05&5\\
SubtropN\_FSDSC&Tropical\_TREFHT&41&6.40E-05&2.90E-05&5\\
Tropical\_AEROD\_v&Tropical\_TREFHT&21&6.40E-05&4.00E-05&5\\
Tropical\_AEROD\_v&Tropical\_FSDSC&26&6.30E-05&3.70E-05&3\\
SubtropN\_AEROD\_v&Tropical\_TREFHT&51&6.00E-05&1.70E-05&5\\
SubtropN\_AEROD\_v&Tropical\_TREFHT&16&6.00E-05&2.30E-05&5\\
Tropical\_FSDSC&Tropical\_TREFHT&6&6.00E-05&3.50E-05&5\\
SubtropN\_FSDSC&Tropical\_FSDSC&21&6.00E-05&4.00E-05&2\\
SubtropN\_AEROD\_v&Tropical\_AEROD\_v&31&6.00E-05&5.20E-05&4\\
SubtropN\_FSDSC&Tropical\_AEROD\_v&31&5.80E-05&8.10E-05&5\\
SubtropN\_TREFHT&Tropical\_FSDSC&6&5.80E-05&6.90E-05&5\\
SubtropN\_TREFHT&Tropical\_TREFHT&51&5.80E-05&3.40E-05&5\\
SubtropN\_AEROD\_v&Tropical\_FSDSC&31&5.80E-05&4.40E-05&5\\
Tropical\_AEROD\_v&SubtropN\_TREFHT&46&5.80E-05&3.20E-05&5\\
SubtropN\_TREFHT&Tropical\_TREFHT&31&5.80E-05&2.60E-05&5\\
Tropical\_TREFHT&Tropical\_AEROD\_v&11&5.70E-05&3.10E-05&3\\
SubtropN\_FSDSC&Tropical\_TREFHT&6&5.70E-05&3.10E-05&3\\
SubtropN\_FSDSC&Tropical\_TREFHT&21&5.60E-05&3.40E-05&5\\
SubtropN\_TREFHT&Tropical\_TREFHT&6&5.60E-05&2.60E-05&5\\
SubtropN\_AEROD\_v&Tropical\_TREFHT&41&5.60E-05&2.90E-05&5\\
SubtropN\_FSDSC&Tropical\_TREFHT&56&5.60E-05&2.90E-05&5\\
SubtropN\_TREFHT&Tropical\_TREFHT&16&5.60E-05&2.90E-05&5\\
SubtropN\_AEROD\_v&Tropical\_FSDSC&16&5.50E-05&6.10E-05&4\\
SubtropN\_TREFHT&Tropical\_AEROD\_v&46&5.50E-05&4.20E-05&4\\
SubtropN\_FSDSC&Tropical\_TREFHT&46&5.40E-05&1.40E-05&5\\
SubtropN\_FSDSC&Tropical\_FSDSC&31&5.40E-05&3.10E-05&5\\
Tropical\_FSDSC&Tropical\_TREFHT&51&5.40E-05&2.90E-05&5\\
Tropical\_FSDSC&Tropical\_TREFHT&21&5.40E-05&3.60E-05&5\\
SubtropN\_AEROD\_v&Tropical\_AEROD\_v&1&5.30E-05&4.20E-05&3\\
Tropical\_AEROD\_v&Tropical\_AEROD\_v&51&5.30E-05&6.30E-05&4\\
Tropical\_AEROD\_v&Tropical\_TREFHT&36&5.20E-05&2.30E-05&5\\
Tropical\_TREFHT&Tropical\_FSDSC&46&5.20E-05&3.50E-05&5\\
Tropical\_AEROD\_v&Tropical\_TREFHT&31&5.00E-05&4.10E-05&4\\
SubtropN\_TREFHT&Tropical\_AEROD\_v&6&5.00E-05&3.10E-05&4\\
Tropical\_AEROD\_v&Tropical\_TREFHT&16&5.00E-05&3.30E-05&5\\
SubtropN\_TREFHT&Tropical\_FSDSC&26&5.00E-05&3.40E-05&4\\
SubtropN\_FSDSC&Tropical\_FSDSC&41&5.00E-05&2.10E-05&4\\
Tropical\_TREFHT&Tropical\_FSDSC&31&5.00E-05&3.70E-05&4\\
Tropical\_TREFHT&Tropical\_FSDSC&21&5.00E-05&5.00E-05&3\\
Tropical\_AEROD\_v&Tropical\_TREFHT&46&5.00E-05&2.80E-05&5\\
SubtropN\_TREFHT&Tropical\_AEROD\_v&56&5.00E-05&8.00E-06&3\\
Tropical\_TREFHT&Tropical\_TREFHT&46&4.80E-05&2.20E-05&5\\
Tropical\_TREFHT&Tropical\_FSDSC&16&4.80E-05&2.30E-05&5\\
Tropical\_TREFHT&Tropical\_FSDSC&6&4.80E-05&4.50E-05&5\\
Tropical\_FSDSC&Tropical\_TREFHT&36&4.80E-05&1.60E-05&5\\
Tropical\_TREFHT&Tropical\_FSDSC&11&4.80E-05&4.80E-05&5\\
SubtropN\_AEROD\_v&Tropical\_AEROD\_v&41&4.70E-05&2.40E-05&3\\
Tropical\_AEROD\_v&Tropical\_TREFHT&1&4.60E-05&2.40E-05&5\\
Tropical\_TREFHT&Tropical\_AEROD\_v&41&4.60E-05&4.40E-05&5\\
SubtropN\_AEROD\_v&Tropical\_TREFHT&56&4.60E-05&1.40E-05&5\\
Tropical\_FSDSC&Tropical\_TREFHT&56&4.50E-05&2.10E-05&4\\
Tropical\_FSDSC&Tropical\_FSDSC&36&4.50E-05&2.50E-05&2\\
Tropical\_AEROD\_v&Tropical\_TREFHT&41&4.40E-05&2.70E-05&5\\
SubtropN\_TREFHT&Tropical\_FSDSC&46&4.30E-05&4.00E-05&3\\
SubtropN\_AEROD\_v&Tropical\_FSDSC&1&4.30E-05&2.30E-05&4\\
Tropical\_TREFHT&Tropical\_FSDSC&36&4.30E-05&1.80E-05&4\\
SubtropN\_FSDSC&Tropical\_AEROD\_v&16&4.30E-05&8.00E-06&4\\
Tropical\_FSDSC&Tropical\_TREFHT&41&4.20E-05&7.00E-06&5\\
Tropical\_AEROD\_v&Tropical\_TREFHT&11&4.20E-05&1.00E-05&5\\
SubtropN\_AEROD\_v&Tropical\_TREFHT&21&4.20E-05&1.60E-05&5\\
Tropical\_FSDSC&Tropical\_FSDSC&31&4.00E-05&1.00E-05&2\\
Tropical\_AEROD\_v&Tropical\_TREFHT&6&4.00E-05&1.40E-05&5\\
Tropical\_TREFHT&Tropical\_AEROD\_v&51&4.00E-05&2.80E-05&3\\
Tropical\_AEROD\_v&Tropical\_AEROD\_v&31&4.00E-05&2.20E-05&3\\
SubtropN\_AEROD\_v&Tropical\_AEROD\_v&26&4.00E-05&2.20E-05&3\\
Tropical\_FSDSC&Tropical\_AEROD\_v&51&4.00E-05&3.00E-05&2\\
Tropical\_TREFHT&Tropical\_AEROD\_v&36&4.00E-05&3.00E-05&2\\
SubtropN\_AEROD\_v&Tropical\_TREFHT&6&4.00E-05&2.20E-05&5\\
SubtropN\_TREFHT&Tropical\_TREFHT&46&3.80E-05&1.60E-05&5\\
Tropical\_FSDSC&Tropical\_TREFHT&26&3.80E-05&1.70E-05&5\\
SubtropN\_FSDSC&Tropical\_AEROD\_v&21&3.80E-05&2.50E-05&4\\
SubtropN\_FSDSC&Tropical\_FSDSC&1&3.80E-05&8.00E-06&4\\
Tropical\_AEROD\_v&Tropical\_FSDSC&51&3.70E-05&2.40E-05&4\\
Tropical\_FSDSC&Tropical\_AEROD\_v&16&3.70E-05&1.20E-05&3\\
SubtropN\_TREFHT&Tropical\_AEROD\_v&41&3.70E-05&3.10E-05&3\\
Tropical\_TREFHT&Tropical\_AEROD\_v&46&3.70E-05&2.50E-05&3\\
SubtropN\_TREFHT&Tropical\_AEROD\_v&26&3.70E-05&3.80E-05&3\\
Tropical\_AEROD\_v&Tropical\_TREFHT&56&3.70E-05&9.00E-06&3\\
SubtropN\_AEROD\_v&Tropical\_AEROD\_v&6&3.70E-05&1.70E-05&3\\
SubtropN\_AEROD\_v&Tropical\_FSDSC&46&3.50E-05&2.10E-05&4\\
Tropical\_FSDSC&Tropical\_AEROD\_v&46&3.50E-05&2.50E-05&2\\
Tropical\_AEROD\_v&Tropical\_AEROD\_v&21&3.50E-05&1.50E-05&4\\
Tropical\_TREFHT&Tropical\_FSDSC&26&3.50E-05&1.10E-05&4\\
SubtropN\_AEROD\_v&Tropical\_FSDSC&21&3.50E-05&2.30E-05&4\\
Tropical\_TREFHT&Tropical\_AEROD\_v&1&3.30E-05&2.10E-05&3\\
SubtropN\_FSDSC&Tropical\_FSDSC&36&3.30E-05&1.70E-05&3\\
Tropical\_FSDSC&Tropical\_AEROD\_v&36&3.30E-05&1.70E-05&3\\
Tropical\_TREFHT&Tropical\_FSDSC&41&3.30E-05&1.60E-05&4\\
Tropical\_TREFHT&Tropical\_AEROD\_v&21&3.20E-05&1.20E-05&5\\
Tropical\_FSDSC&Tropical\_FSDSC&6&3.20E-05&2.20E-05&5\\
Tropical\_FSDSC&Tropical\_TREFHT&11&3.00E-05&1.40E-05&5\\
Tropical\_FSDSC&Tropical\_TREFHT&31&3.00E-05&1.40E-05&5\\
Tropical\_FSDSC&Tropical\_FSDSC&46&3.00E-05&2.00E-05&2\\
SubtropN\_FSDSC&Tropical\_FSDSC&6&3.00E-05&1.60E-05&4\\
Tropical\_AEROD\_v&Tropical\_AEROD\_v&56&3.00E-05&2.20E-05&3\\
SubtropN\_TREFHT&Tropical\_FSDSC&16&2.80E-05&1.80E-05&5\\
SubtropN\_TREFHT&Tropical\_AEROD\_v&31&2.80E-05&1.90E-05&5\\
SubtropN\_TREFHT&Tropical\_FSDSC&56&2.80E-05&1.30E-05&4\\
Tropical\_FSDSC&Tropical\_FSDSC&51&2.80E-05&2.00E-05&4\\
Tropical\_FSDSC&Tropical\_AEROD\_v&41&2.80E-05&1.90E-05&4\\
SubtropN\_AEROD\_v&Tropical\_FSDSC&36&2.80E-05&8.00E-06&4\\
Tropical\_FSDSC&Tropical\_FSDSC&56&2.70E-05&1.20E-05&3\\
SubtropN\_FSDSC&Tropical\_AEROD\_v&36&2.70E-05&1.70E-05&3\\
SubtropN\_FSDSC&Tropical\_FSDSC&11&2.60E-05&1.60E-05&5\\
Tropical\_FSDSC&Tropical\_AEROD\_v&11&2.50E-05&1.10E-05&4\\
Tropical\_AEROD\_v&Tropical\_AEROD\_v&11&2.50E-05&5.00E-06&4\\
SubtropN\_TREFHT&Tropical\_AEROD\_v&51&2.50E-05&1.50E-05&4\\
SubtropN\_AEROD\_v&Tropical\_FSDSC&6&2.40E-05&1.00E-05&5\\
SubtropN\_TREFHT&Tropical\_FSDSC&11&2.40E-05&1.90E-05&5\\
Tropical\_TREFHT&Tropical\_AEROD\_v&56&2.30E-05&9.00E-06&3\\
SubtropN\_AEROD\_v&Tropical\_AEROD\_v&51&2.30E-05&5.00E-06&3\\
SubtropN\_FSDSC&Tropical\_AEROD\_v&11&2.30E-05&1.20E-05&3\\
SubtropN\_TREFHT&Tropical\_FSDSC&41&2.30E-05&1.10E-05&4\\
Tropical\_FSDSC&Tropical\_FSDSC&16&2.30E-05&1.60E-05&4\\
Tropical\_AEROD\_v&Tropical\_FSDSC&56&2.00E-05&0.00E+00&2\\
SubtropN\_AEROD\_v&Tropical\_AEROD\_v&36&2.00E-05&8.00E-06&3\\
Tropical\_TREFHT&Tropical\_FSDSC&51&2.00E-05&8.00E-06&3\\
Tropical\_AEROD\_v&Tropical\_FSDSC&16&2.00E-05&0.00E+00&1\\
SubtropN\_FSDSC&Tropical\_AEROD\_v&6&2.00E-05&1.00E-05&2\\
Tropical\_AEROD\_v&Tropical\_AEROD\_v&26&2.00E-05&1.20E-05&4\\
SubtropN\_FSDSC&Tropical\_FSDSC&16&2.00E-05&0.00E+00&3\\
Tropical\_TREFHT&Tropical\_AEROD\_v&16&2.00E-05&7.00E-06&4\\
Tropical\_AEROD\_v&Tropical\_FSDSC&11&2.00E-05&0.00E+00&1\\
Tropical\_TREFHT&Tropical\_AEROD\_v&26&2.00E-05&0.00E+00&1\\
Tropical\_AEROD\_v&Tropical\_FSDSC&41&2.00E-05&0.00E+00&2\\
SubtropN\_AEROD\_v&Tropical\_AEROD\_v&11&2.00E-05&0.00E+00&3\\
SubtropN\_AEROD\_v&Tropical\_FSDSC&56&1.80E-05&1.20E-05&5\\
SubtropN\_FSDSC&Tropical\_AEROD\_v&51&1.80E-05&7.00E-06&5\\
SubtropN\_TREFHT&Tropical\_AEROD\_v&36&1.80E-05&1.30E-05&4\\
Tropical\_TREFHT&Tropical\_AEROD\_v&31&1.80E-05&8.00E-06&4\\
SubtropN\_FSDSC&Tropical\_AEROD\_v&1&1.70E-05&9.00E-06&3\\
SubtropN\_FSDSC&Tropical\_AEROD\_v&41&1.60E-05&8.00E-06&5\\
SubtropN\_TREFHT&Tropical\_AEROD\_v&11&1.50E-05&5.00E-06&2\\
SubtropN\_FSDSC&Tropical\_AEROD\_v&46&1.50E-05&5.00E-06&2\\
SubtropN\_FSDSC&Tropical\_FSDSC&56&1.50E-05&5.00E-06&2\\
SubtropN\_FSDSC&Tropical\_FSDSC&51&1.50E-05&5.00E-06&2\\
Tropical\_AEROD\_v&Tropical\_AEROD\_v&41&1.30E-05&5.00E-06&3\\
SubtropN\_AEROD\_v&Tropical\_AEROD\_v&56&1.30E-05&5.00E-06&3\\
SubtropN\_AEROD\_v&Tropical\_FSDSC&51&1.30E-05&5.00E-06&3\\
SubtropN\_FSDSC&Tropical\_AEROD\_v&56&1.30E-05&5.00E-06&3\\
Tropical\_AEROD\_v&Tropical\_AEROD\_v&6&1.30E-05&5.00E-06&3\\
Tropical\_AEROD\_v&Tropical\_FSDSC&46&1.30E-05&5.00E-06&3\\
SubtropN\_AEROD\_v&Tropical\_FSDSC&11&1.30E-05&5.00E-06&3\\
SubtropN\_TREFHT&Tropical\_AEROD\_v&16&1.30E-05&4.00E-06&4\\
Tropical\_AEROD\_v&Tropical\_AEROD\_v&46&1.00E-05&0.00E+00&1\\
SubtropN\_AEROD\_v&Tropical\_AEROD\_v&46&1.00E-05&0.00E+00&1\\
\hline
\end{longtblr}
